# Supplementary material for: Floating flocks: Two-dimensional long-range uniaxial order in three-dimensional active fluids
Source: arXiv:2110.15633 ancillary file (2023-01-13)
Supplement: Supplementary file 2 [file film_nem_ch_Supp_arxiv.pdf]

# Floating flocks: Two-dimensional long-range uniaxial order in three-dimensional active fluids

## Supplementary Material

Ananyo Maitra<sup>1,2,\*</sup>

<sup>1</sup>*Laboratoire de Physique Théorique et Modélisation, CNRS UMR 8089,  
CY Cergy Paris Université, F-95302 Cergy-Pontoise Cedex, France*

<sup>2</sup>*Sorbonne Université and CNRS, Laboratoire Jean Perrin, F-75005, Paris, France*

In this supplement, I present the detailed calculations for the results discussed in the main paper. I show that the density fluctuations do not affect the orientational fluctuations (in the hydrodynamic limit) when there is a particle exchange between the bulk fluid and the interface (NNC and PNC models) in Sec. A. In Sec B, I present a detailed derivation of the effective interfacial or surface velocity field. In Sec. C, I calculate the noises that appear in the director dynamics stemming from its coupling to bulk fluid flow. In Sec. D, I describe the four models considered in the main text in more detail. Sec. E contains a detailed demonstration of long-range interfacial order in the NNC models (i.e., interfacial nematic with bulk particle exchange). Sec. F demonstrates that nematic interfacial order is possible even in a confined geometry where hydrodynamic interactions are cut-off at the scale of the confinement width. In Sec. G, I present an argument for defect interactions in this interfacial ordered phase being stronger than equilibrium nematics. Sec. H demonstrates that polar order in the PNC model is long-ranged. Sec. I displays the subdominant corrections to the equations for angular fluctuations in both the PNC and NNC models. Sec. J details the calculations demonstrating that an ordered phase is generally impossible in the NC model. In Sec. K, I demonstrate that a stable nematic phase is possible in NC model but only when a special relation is satisfied between the coefficients. In Sec. L, I describe the instability of *bulk* nematic phases in *compressible*, momentum-conserved active fluids and show that it is reminiscent of the instability of the NC model discussed in Sec. J. I display the detailed calculations demonstrating that highly motile polar flocks exist even when the flocers are confined to a fluid surface or interface (PC model) in Sec. M. Sec. N considers the effects of interfacial (surface) fluctuations on the interface-associated (surface-associated) ordered phase.

### Appendix A: Demonstration that interfacial concentration in NNC and PNC models are not hydrodynamic

In this supplementary section, I demonstrate that the interfacial concentration of active particles is not a hydrodynamic variable, and does not affect the long-time, large-scale properties of the interfacial ordered phase, in the NNC and the PNC models (i.e., when the active particles can move between the bulk and the interface).

I take the concentration of active particles, or in the case of active polymers formed from monomers, the concentration of monomers in the polymeric state, at the interface or the boundary to be  $c(\mathbf{r}_\perp, t)$ , where  $\mathbf{r}_\perp \equiv (x, y)$ . The concentration of active particles or monomers in the bulk is  $\rho(\mathbf{r}, t)$  with  $\mathbf{r} \equiv (x, y, z)$ . The total number of active particles, or monomers composing active particles,  $\int d\mathbf{r}_\perp [c + \int dz \rho] = N_{\text{tot}}$  in the system is constant. For a surface-associated nematic phase at the boundary of a semi-infinite fluid,  $\rho$  diffuses in the bulk below the interface. Even for an interface between two fluids, I assume that  $\rho$  only diffuses in the fluid below the interface. This assumption can be easily relaxed and the argument presented here works even when the particles diffuse in the fluids both above and below the interface. The bulk density  $\rho$  is conserved inside the fluid and gets converted to  $c$  only at the boundary. Therefore, in the bulk,  $\rho$  obeys a conservation equation of the form

$$\partial_t \rho + \mathbf{V}_b \cdot \nabla \rho = D_\rho \nabla^2 \rho \quad (\text{A1})$$

with a boundary condition at the surface of the bulk fluid  $z = 0$ ,  $D_\rho \partial_z \rho|_{z=0} = j$  where  $j$  is the flux of  $\rho$  into and out of the bulk. The surface concentration field  $c$  has an equation of motion [1, 2]

$$\partial_t c = -\nabla_\perp \cdot (c\mathbf{v}) - \nabla_\perp \cdot \mathbf{J}^a + D_c \nabla_\perp^2 c + j \quad (\text{A2})$$

where  $\mathbf{J}^a$  is the active current which, for a nematic system, has the form  $\mathbf{J}^a = g_{Q1}(c)\nabla_\perp \cdot [g_{Q2}(c)\mathbf{Q}]$  where  $g_{Q1}(c)$  and  $g_{Q2}(c)$  are arbitrary functions of the concentration and  $j$  is the flux of particles into and out of the interface. Eqs. (A1) along with its boundary condition and (A2) together imply that there is an exchange of particles between the bulk fluid and the surface. The flux  $j$  is generally modelled as [1, 2]

$$j = k_a \rho|_{z=0} \left(1 - \frac{c}{c_{\text{max}}}\right) - k_d c \quad (\text{A3})$$

where  $k_a$  is the adsorption rate,  $k_d$  is the desorption rate,  $c_{\max}$  is the maximum interfacial concentration and  $\rho|_{z=0}$  is the bulk density adjacent to the interface. The specific form of  $j$  is unimportant; it simply models the adsorption and desorption of the particles to and from the interface.

In the steady state,  $\rho = \rho_0$  everywhere and  $j = 0$  implying that  $c_0 = k_a \rho_0 c_{\max} / (k_d c_{\max} + k_a \rho_0)$ . Eq. (A2) along with (A3) imply that deviations of  $\delta c$  of  $c$  from this steady-state value are not hydrodynamic but relax at a finite time as

$$\partial_t \delta c = k_a \delta \rho|_{z=0} - \frac{k_a}{c_{\max}} \rho_0 \delta c - k_d \delta c. \quad (\text{A4})$$

This implies that  $\delta c$  adjusts in a finite time to preserve  $j = 0$  and is slaved to the fluctuations of the bulk density adjacent to the interface via

$$\delta c = \frac{c_{\max} k_a}{k_a \rho_0 + k_d c_{\max}} \delta \rho|_{z=0}. \quad (\text{A5})$$

The bulk fluid in the NNC model, therefore, acts as a reservoir for the concentration of the particles at the interface, and this concentration, therefore, is not globally conserved, but locally fixed – a local excess or deficit of  $c$  decays primarily by the exchange with the bulk, i.e., by diffusion into or out of the bulk fluid, and not by diffusion within the boundary layer. Further, since  $j$  relaxes to 0 in a finite time, the bulk density field (A1) effectively has a no-flux condition at the interface and, to linear order, is not affected by fluctuations of either the velocity field or the order parameter field. That is, it relaxes independently of other fields.

Furthermore, the stochastic part of  $\delta c$  only contributes noises in the order parameter equations that are irrelevant compared to the noise already present in that equation. This fluctuating part can be obtained by introducing noises in both (A1) and (A2). To the lowest order in gradients, the noise in (A2) is a non-conserving noise in  $j$ . This implies that  $\delta c$  has a stochastic part whose standard deviation doesn't vanish at small wavenumbers. However, by symmetry,  $\delta c$  can only enter order parameter equations with one power of wavenumber and, therefore, the effect of this noise on the order parameter dynamics is subdominant to the wavenumber-independent noise already present in that equation. Eq. (A1) has a bulk, conserving noise. This implies that the *zero-frequency weight* of the noise affecting  $\delta c$  through its coupling to  $\delta \rho|_{z=0}$  is  $\propto 1/|q_{\perp}|$ . Again, since  $\delta c$  only enters order parameter equations with one power of wavenumber, the effect of even this noise is subdominant to the non-conserving noise present there. Therefore, I can also safely ignore the stochastic fluctuations due to  $\delta c$ . This completes the demonstration that  $\delta c$  can be disregarded in the NNC and PNC models.

The bulk fluid equation has a contribution from the bulk density of the form  $-\rho \nabla \delta F_{\rho} / \delta \rho$  where  $F_{\rho}$  is the bulk free energy of the particles. The linearised force due to density fluctuations is, therefore,  $-\rho_0 \nabla \delta F_{\rho} / \delta \rho$  which can be absorbed into a redefinition of the pressure  $\Pi_b$ . There are possible active forces involving  $\rho$  of the form  $\nabla \cdot (\nabla \rho \nabla \rho)$  [3–5] but in a homogeneous state, these again lead to conserving noises which vanish faster at small wavenumbers than the noise considered in Sec. C and is, therefore, even less relevant. This implies that bulk density fluctuations do not affect the hydrodynamics of interfacial order in the PNC and NNC models as well. Further, this part of the argument is completely independent of the interconversion between  $\rho$  and  $c$  at the boundary. Therefore, this argument also means that bulk density fluctuations do not affect the hydrodynamics of interfacial order in the PC and NC models as well.

## Appendix B: Detailed derivation of the mobility for the calculation of interfacial velocity field in terms of the interfacial forces

In this supplementary section, I present the detailed steps required to obtain the mobility tensor used in the main text (see Eq. (3) of the main text). I consider an interface between two incompressible fluids with viscosity  $\eta_t$  and  $\eta_b$ . The fluids above and below the interface support no uniaxial order even when active units dissolve in the bulk fluid, irrespective of the bulk density of the active units [6]. This is due to the instability of the bulk active nematic which implies that the active units essentially lead to a conserving noise correlated over finite spatial and temporal scales [7, 8]. As shown in Supp. C, such noises in the bulk fluids above and below the interface do not modify the hydrodynamic behaviour of the interfacial ordered state and, therefore, I neglect them here. With these considerations, the Stokes equations for the fluid velocities above and below the interface,  $\mathbf{V}_t$  and  $\mathbf{V}_b$  respectively, are

$$\eta_t \nabla^2 \mathbf{V}_t = \nabla \Pi_t \quad (\text{B1})$$

and

$$\eta_b \nabla^2 \mathbf{V}_b = \nabla \Pi_b \quad (\text{B2})$$

where  $\eta_t$  and  $\eta_b$  are the viscosities of the fluids above and below the interface respectively and the pressures  $\Pi_t$  and  $\Pi_b$  are determined by the incompressibility constraints  $\nabla \cdot \mathbf{V}_t = 0$  and  $\nabla \cdot \mathbf{V}_b = 0$ . The incompressibility constraint implies that  $\nabla^2 \Pi_t = \nabla^2 \Pi_b = 0$  and  $\nabla^4 \mathbf{V}_t = \nabla^4 \mathbf{V}_b = 0$ . Fourier transforming in the  $x$  and  $y$  directions, transverse to the interface, the latter yields

$$(q_\perp^4 + \partial_z^4 - 2q_\perp^2 \partial_z^2) \mathbf{V}_{tq}(z) = 0, \quad (\text{B3})$$

and

$$(q_\perp^4 + \partial_z^4 - 2q_\perp^2 \partial_z^2) \mathbf{V}_{bq}(z) = 0. \quad (\text{B4})$$

These equations have to be solved with boundary conditions  $\mathbf{V}_{tq}(0) = \mathbf{V}_{bq}(0) = \mathbf{v}$ , where  $\mathbf{v}$  is the interfacial velocity, and  $\lim_{z \rightarrow \infty} \mathbf{V}_{tq}(z) \rightarrow 0$  and  $\lim_{z \rightarrow -\infty} \mathbf{V}_{bq}(z) \rightarrow 0$ . The general solutions of this form are

$$\mathbf{V}_{tq}(z) = e^{-|q_\perp|z} (\mathbf{v} + z\mathbf{T}) \quad (\text{B5})$$

and

$$\mathbf{V}_{bq}(z) = e^{|q_\perp|z} (\mathbf{v} + z\mathbf{B}) \quad (\text{B6})$$

where  $\mathbf{T}$  and  $\mathbf{B}$  are  $\mathbf{q}_\perp$ -dependent quantities which have to be determined. Taking the curl of (B1) and (B2) and using these solutions yield

$$(i\mathbf{q}_\perp + \partial_z \hat{z}) \times (-q_\perp^2 + \partial_z^2) \mathbf{V}_{tq}(z) = 0 \implies (-|q_\perp| \hat{z} + i\mathbf{q}_\perp) \times \mathbf{T} = 0 \implies \mathbf{q}_\perp \times \mathbf{T}_\perp = 0 \quad (\text{B7})$$

and similarly,

$$(|q_\perp| \hat{z} + i\mathbf{q}_\perp) \times \mathbf{B} = 0 \implies \mathbf{q}_\perp \times \mathbf{B}_\perp = 0 \quad (\text{B8})$$

i.e., both  $\mathbf{T}_\perp$  and  $\mathbf{B}_\perp$  must be vectors parallel to  $\mathbf{q}_\perp$ . Taking the divergence of the velocity fields yield

$$(i\mathbf{q}_\perp \cdot \mathbf{v} + T_z) + (i\mathbf{q}_\perp \cdot \mathbf{T}_\perp - T_z |q_\perp|)z = 0 \quad (\text{B9})$$

and

$$(i\mathbf{q}_\perp \cdot \mathbf{v} + B_z) + (i\mathbf{q}_\perp \cdot \mathbf{B}_\perp + B_z |q_\perp|)z = 0. \quad (\text{B10})$$

This implies that  $T_z = -i\mathbf{q}_\perp \cdot \mathbf{v}$ ,  $B_z = -i\mathbf{q}_\perp \cdot \mathbf{v}$  and

$$\mathbf{q}_\perp \cdot \mathbf{T}_\perp = -\mathbf{q}_\perp \cdot \mathbf{v} |q_\perp| \implies \mathbf{T}_\perp = -\frac{\mathbf{q}_\perp \mathbf{q}_\perp}{|q_\perp|} \cdot \mathbf{v}, \quad (\text{B11})$$

where I have used the fact that  $\mathbf{T}_\perp$  is a vector parallel to  $\mathbf{q}_\perp$  in the last step. Similarly,  $\mathbf{B}_\perp = \mathbf{q}_\perp \mathbf{q}_\perp \cdot \mathbf{v} / |q_\perp|$ . Therefore, the velocity fields at the top and the bottom of the interface, in terms of the interfacial velocity field, are

$$\mathbf{V}_{tq}(z) = e^{-|q_\perp|z} [\mathbf{v} - z(i\hat{z} - \hat{q}_\perp)(\mathbf{q}_\perp \cdot \mathbf{v})] \quad (\text{B12})$$

and

$$\mathbf{V}_{bq}(z) = e^{|q_\perp|z} [\mathbf{v} - z(i\hat{z} - \hat{q}_\perp)(\mathbf{q}_\perp \cdot \mathbf{v})]. \quad (\text{B13})$$

Eqs. (B12) and (B13) imply that while  $\nabla \cdot \mathbf{V}_b = \nabla \cdot \mathbf{V}_t = 0$ ,  $\nabla_\perp \cdot \mathbf{v} \neq 0$ , i.e., the interfacial flow is not itself incompressible with compressional or dilational in-plane flows balanced by  $\partial_z(V_t)_z$  and  $\partial_z(V_b)_z$  at  $z = 0$ . These equations further imply that

$$\partial_z \mathbf{V}_{tq}|_{z=0} = -\frac{q_\perp^2 \mathbf{I} + \mathbf{q}_\perp \mathbf{q}_\perp}{|q_\perp|} \cdot \mathbf{v} - i\mathbf{q}_\perp \cdot \mathbf{v} \hat{z} \quad (\text{B14})$$

and

$$\partial_z \mathbf{V}_{bq}|_{z=0} = \frac{q_\perp^2 \mathbf{I} + \mathbf{q}_\perp \mathbf{q}_\perp}{|q_\perp|} \cdot \mathbf{v} - i\mathbf{q}_\perp \cdot \mathbf{v} \hat{z}, \quad (\text{B15})$$

where  $\mathbf{I}$  is the  $2 \times 2$  identity matrix and the  $\hat{z}$  component could have been directly obtained from the three-dimensional incompressibility constraint and the fact that  $\mathbf{V}_{tq}(z=0) = \mathbf{V}_{bq}(z=0) = \mathbf{v}$ .

Eqs. (B14) and (B15) directly yield the difference of the tangential stresses between the top and the bottom fluid at  $z=0$  which has to be balanced by the surface forces. Separating out the interfacial viscous forces from those arising due to interfacial director distortions and concentration fluctuations of the ordered active species and writing the latter as  $\mathbf{f}^s = i\mathbf{q}_\perp \cdot \boldsymbol{\sigma}^s$ , where  $\boldsymbol{\sigma}^s$  is the interfacial particle-phase stress, I get

$$\eta_t \partial_z (\mathbf{V}_{tq})_\perp|_{z=0} - \eta_b \partial_z (\mathbf{V}_{bq})_\perp|_{z=0} - \eta_{ss} q_\perp^2 \mathbf{v} - \eta_{sb} \mathbf{q}_\perp (\mathbf{q}_\perp \cdot \mathbf{v}) = -i\mathbf{q}_\perp \cdot \boldsymbol{\sigma}^s. \quad (\text{B16})$$

Defining  $\eta = (\eta_t + \eta_b)/2$  and the Saffmann-Delbrück lengths [9]  $\ell_s = \eta_{ss}/2\eta$  and  $\ell_b = \eta_{sb}/2\eta$ , I obtain an expression of the in-plane velocity fields in terms of the in-plane particle-phase stress or force in the form  $\mathbf{v} = i\mathbf{M} \cdot (\mathbf{q}_\perp \cdot \boldsymbol{\sigma}^s) = \mathbf{M} \cdot \mathbf{f}^s$  with a mobility

$$\mathbf{M} = \frac{1}{2\eta|q_\perp|^3[2 + (\ell_b + 3\ell_s)|q_\perp| + \ell_s(\ell_b + \ell_s)q_\perp^2]} \begin{pmatrix} q_x^2(1 + \ell_s|q_\perp|) + q_y^2[2 + (\ell_s + \ell_b)|q_\perp|] & -q_x q_y(1 + \ell_b|q_\perp|) \\ -q_x q_y(1 + \ell_b|q_\perp|) & q_y^2(1 + \ell_s|q_\perp|) + q_x^2[2 + (\ell_s + \ell_b)|q_\perp|] \end{pmatrix}. \quad (\text{B17})$$

For in-plane scales larger than the Saffmann-Delbrück ones, i.e., when  $\ell_s|q_\perp|, \ell_b|q_\perp| \ll 1$ , that is relevant for the hydrodynamic theory of an interfacial ordered state, this reduces to

$$\mathbf{M} = \frac{1}{4\eta|q_\perp|^3} \begin{pmatrix} q_x^2 + 2q_y^2 & -q_x q_y \\ -q_x q_y & 2q_x^2 + q_y^2 \end{pmatrix} - \frac{1}{8\eta q_\perp^2} \begin{pmatrix} (\ell_b + \ell_s)q_x^2 + 4\ell_s q_y^2 & (\ell_b - 3\ell_s)q_x q_y \\ (\ell_b - 3\ell_s)q_x q_y & (\ell_b + \ell_s)q_y^2 + 4\ell_s q_x^2 \end{pmatrix} + \mathcal{O}(\ell_b^2, \ell_s^2, \ell_s \ell_b) \quad (\text{B18})$$

Thus, it is clear that the surface viscosities, through  $\ell_b$  and  $\ell_s$ , lead to higher order in wavenumber corrections to the mobility which are irrelevant for the hydrodynamic properties of the ordered state. Further, an equivalent calculation of the mobility can be performed when there is no fluid above the interface i.e., no equation for  $\mathbf{V}_t$ . This describes the behaviour of a phase associated with the stress-free boundary of a semi-infinite bulk fluid. In this case, the effective mobility is still given by (B17) but with an effective viscosity  $\eta = \eta_b/2$ . Therefore, (B17) can be used to obtain the velocity field at the interface between two fluids, at an air-fluid interface and at an immersed surface – such as a membrane – in a bulk fluid simply by modifying the definition of the parameter  $\eta$ :  $\eta = (\eta_t + \eta_b)/2$  in the first case,  $\eta = \eta_b/2$  in the second and  $\eta = \eta_f$ , where  $\eta_f$  is the viscosity of the bulk fluid, in the third.

### Appendix C: Noise stemming from the velocity coupling in the angle and concentration equations

In this supplementary section, I will calculate the noises that enter the angle field equation and the concentration equation due to the coupling with the velocity field. The Stokes equation has a conserving noise that I ignored in the main paper. I will now show that it is irrelevant. For simplicity, I will consider an immersed interface in a fluid with the same value of viscosity both above and below the interface. As mentioned in the main text and discussed more fully in Supp. B, to obtain the results for an interface between two dissimilar fluids or an air-fluid boundary one only needs to change the viscosity to an effective viscosity. I first consider a spatiotemporally uncorrelated noise in the velocity equation. The Stokes equation for the bulk three-dimensional fluid is

$$-\eta \nabla^2 \mathbf{V} = -\nabla \Pi + \mathbf{f}^s \delta(z) + \boldsymbol{\xi}^v, \quad (\text{C1})$$

where  $\mathbf{f}^s$  is the surface force density, the noise  $\boldsymbol{\xi}^v$  has the correlation  $\langle \boldsymbol{\xi}^v(\mathbf{r}, t) \boldsymbol{\xi}^v(\mathbf{r}', t') \rangle = -2\Delta^v \mathbf{I} \nabla^2 \delta(\mathbf{r} - \mathbf{r}') \delta(t - t')$  and I have suppressed the in-plane viscosities (i.e., effectively assumed that the Saffmann-Delbrück lengths are 0; see Supp. B). Retaining in-plane viscosity would ultimately lead to noise contributions in the equations for the in-plane order parameter and concentration that vanish even more strongly at small wavenumber and, thus, are even less relevant. The in-plane velocity fields at  $z=0$ , including the stochastic part, are obtained by eliminating the pressure  $\Pi$  by projecting (C1) transverse to the wavevector, using the three-dimensional transverse projector in the Fourier space,  $\mathcal{P}_{ij} = \delta_{ij} - q_i q_j / q^2$  and integrating the velocity field  $\mathbf{V}$  over all  $q_z$ :

$$v_x = \int_{-\infty}^{\infty} \frac{dq_z}{2\pi} \frac{-f_y^s q_x q_y + f_x^s (q_y^2 + q_z^2)}{\eta q^4} + \int_{-\infty}^{\infty} \frac{dq_z}{2\pi} \frac{1}{\eta q^4} [q_x (\xi_y^v q_y + \xi_z^v q_z) - \xi_x^v (q_y^2 + q_z^2)] = \frac{f_x^s (q_x^2 + 2q_y^2) - f_y^s q_x q_y}{4\eta |q_\perp|^3} + \bar{\xi}_x^v, \quad (\text{C2})$$

$$v_y = \int_{-\infty}^{\infty} \frac{dq_z}{2\pi} \frac{-f_x^s q_x q_y + f_y^s (q_x^2 + q_z^2)}{\eta q^4} + \int_{-\infty}^{\infty} \frac{dq_z}{2\pi} \frac{1}{\eta q^4} [q_y (\xi_x^v q_x + \xi_z^v q_z) - \xi_y^v (q_x^2 + q_z^2)] = \frac{f_y^s (q_x^2 + 2q_y^2) - f_x^s q_x q_y}{4\eta |q_\perp|^3} + \bar{\xi}_y^v, \quad (\text{C3})$$

and

$$V_z|_{(z=0)} = - \int_{-\infty}^{\infty} \frac{dq_z}{2\pi} \frac{q_z \mathbf{q}_{\perp} \cdot \mathbf{f}^s}{\eta q^4} + \int_{-\infty}^{\infty} \frac{dq_z}{2\pi} \frac{1}{\eta q^4} [q_z (\xi_x^v q_x + \xi_y^v q_y) - \xi_z^v q_{\perp}^2] = \bar{\xi}_z^v, \quad (\text{C4})$$

where  $\mathbf{q}_{\perp} \equiv (q_x, q_y)$  and  $\mathbf{q} \equiv (\mathbf{q}_{\perp}, q_z)$ . The correlations of the noises in these equations are

$$\langle \bar{\xi}_x^v(\mathbf{q}_{\perp}, t) \bar{\xi}_x^v(\mathbf{q}'_{\perp}, t') \rangle = \frac{2\Delta^v(q_x^2 + 2q_y^2)}{4\eta^2|q_{\perp}|^3} \delta(\mathbf{q}_{\perp} + \mathbf{q}'_{\perp}) \delta(t - t'), \quad (\text{C5})$$

$$\langle \bar{\xi}_y^v(\mathbf{q}_{\perp}, t) \bar{\xi}_y^v(\mathbf{q}'_{\perp}, t') \rangle = \frac{2\Delta^v(2q_x^2 + q_y^2)}{4\eta^2|q_{\perp}|^3} \delta(\mathbf{q}_{\perp} + \mathbf{q}'_{\perp}) \delta(t - t'), \quad (\text{C6})$$

$$\langle \bar{\xi}_x^v(\mathbf{q}_{\perp}, t) \bar{\xi}_y^v(\mathbf{q}'_{\perp}, t') \rangle = -\frac{2\Delta^v q_x q_y}{4\eta^2|q_{\perp}|^3} \delta(\mathbf{q}_{\perp} + \mathbf{q}'_{\perp}) \delta(t - t'), \quad (\text{C7})$$

$$\langle \bar{\xi}_z^v(\mathbf{q}_{\perp}, t) \bar{\xi}_z^v(\mathbf{q}'_{\perp}, t') \rangle = \frac{2\Delta^v}{4\eta^2|q_{\perp}|} \delta(\mathbf{q}_{\perp} + \mathbf{q}'_{\perp}) \delta(t - t'). \quad (\text{C8})$$

with cross-correlations between  $\bar{\xi}_x^v$  or  $\bar{\xi}_y^v$  and  $\bar{\xi}_z^v$  being 0. This implies that the noise  $\bar{\xi}$  that enters the angle equation via the velocity coupling  $\Omega_{xy} - \lambda A_{xy}$  has the correlation

$$\langle \bar{\xi}(\mathbf{q}_{\perp}, t) \bar{\xi}(\mathbf{q}'_{\perp}, t') \rangle = \frac{2\Delta^v[q_x^4(\lambda - 1)^2 + q_y^4(\lambda + 1)^2 + 2q_x^2 q_y^2]}{8\eta^2|q_{\perp}|^3} \delta(\mathbf{q}_{\perp} + \mathbf{q}'_{\perp}) \delta(t - t') \sim \mathcal{O}(q_{\perp}) \quad (\text{C9})$$

This vanishes at small  $q_{\perp}$ , in all directions and, therefore, it is subdominant to the non-conserving noise in the angle field equation  $\xi$  that is retained in the main paper. This also implies that interfacial *passive* nematic order cannot be facilitated by an active but isotropic interfacial force density, unlike in bulk fluids [10].

The noise  $\bar{\xi}_c$  that enters the concentration equation due to the velocity coupling  $\propto -c_0 \nabla_{\perp} \cdot \mathbf{v}$  has the correlation

$$\langle \bar{\xi}_c(\mathbf{q}_{\perp}, t) \bar{\xi}_c(\mathbf{q}'_{\perp}, t') \rangle = \frac{2c_0^2 \Delta^v |q_{\perp}|}{4\eta^2} \delta(\mathbf{q}_{\perp} + \mathbf{q}'_{\perp}) \delta(t - t'). \quad (\text{C10})$$

This vanishes only as  $|q_{\perp}|$  and is, therefore, more important than the usual conserving noise in the concentration equation which vanishes as  $q_{\perp}^2$  in the small wavenumber limit. Nevertheless, the active couplings to either the nematic or the polar order parameter contribute an anisotropic noise whose zero-frequency weight, when it enters the concentration equation, is  $\sim q_{\perp}^0$ . This can be seen by the following power counting argument:  $-i\omega\delta c \sim iq_{\perp}\theta = -q_{\perp}(i\omega)\theta/\omega$ . Now, the  $\theta$  dynamics has a noise,  $\xi$ , whose strength doesn't vanish at zero wavenumber. Since  $-i\omega\theta \sim \xi$ ,  $-i\omega\delta c \sim -(q_{\perp}/\omega)\xi$ . I will show that both real and imaginary parts of all eigenfrequencies in this work scale as  $\sim q_{\perp}$ . Therefore, the correlator of  $(q_{\perp}/\omega)\xi$  scales the same way (with  $q_{\perp}$  and  $\omega$ ) as  $\xi$  itself; in particular, both scale as  $q_{\perp}^0$  at small wavenumbers. Therefore,  $\bar{\xi}_c$  is subdominant to the noise that appears in the concentration equation via its coupling to the order parameter. In Supp. M, I again explicitly demonstrate that the noise  $\bar{\xi}_c$  does not modify the small wavenumber behaviour of the static structure factor of either the concentration or the order parameter fluctuations.

However, the noises stemming from active stress fluctuations in the bulk fluid (in the spatiotemporally chaotic state) are generically correlated over an active timescale  $\tau_a$  i.e.,  $\langle \xi^v(\mathbf{q}, \omega) \xi^v(\mathbf{q}', \omega') \rangle = 2\Delta^v \mathbf{l} q^2 \delta(\mathbf{q} + \mathbf{q}') \delta(\omega + \omega') / (\tau_a^2 \omega^2 + 1)$ . In this case, the noise stemming from the velocity field in the orientation equation becomes

$$\langle \bar{\xi}(\mathbf{q}_{\perp}, \omega) \bar{\xi}(\mathbf{q}'_{\perp}, \omega') \rangle = \frac{2\Delta^v[q_x^4(\lambda - 1)^2 + q_y^4(\lambda + 1)^2 + 2q_x^2 q_y^2]}{8\eta^2|q_{\perp}|^3(\tau_a^2 \omega^2 + 1)} \delta(\mathbf{q}_{\perp} + \mathbf{q}'_{\perp}) \delta(\omega + \omega') \quad (\text{C11})$$

Even this coloured noise doesn't qualitatively modify the angular fluctuations. Writing the relaxation rate of angular fluctuations in (6) of the main text as  $-\kappa(\phi)|q_{\perp}|$ , the static structure factor of angular fluctuations becomes

$$\langle |\theta(\mathbf{q}_{\perp}, t)|^2 \rangle = \frac{\Delta}{\kappa(\phi)|q_{\perp}|} + \frac{\Delta^v[q_x^4(\lambda - 1)^2 + q_y^4(\lambda + 1)^2 + 2q_x^2 q_y^2]}{8\eta^2|q_{\perp}|^4 \kappa(\phi) [1 + \tau_a |q_{\perp}| \kappa(\phi)]} \quad (\text{C12})$$

For  $\tau_a |q_{\perp}| \kappa(\phi) \ll 1$ , which is *always* realised for small enough  $|q_{\perp}|$  (since  $\kappa(\phi) > 0$  for all  $\phi$  for stable interfacial order), the second term does not diverge at small  $|q_{\perp}|$  unlike the first one. Therefore, it can be neglected in comparison to the first implying that bulk active fluctuations are irrelevant for the hydrodynamic properties of the interfacial phase. Spatially correlated active noises can also be treated the same way and also turn out to be irrelevant. Similar considerations apply to the noise in the concentration equation  $\bar{\xi}_c$ .

## Appendix D: Detailed description of the models

In this supplementary section, I describe the four models I consider, *viz.* the NNC (nematic, non-conserved), PNC (polar, non-conserved), NC (nematic, conserved) and PC (polar, conserved) models, in full detail.

### 1. NNC Model: Interfacial active nematic composed of nematogens diffusing in the bulk

I describe a nematic phase at a fluid-fluid or fluid-air interface with the active particles diffusing in the bulk. The nematogens are constrained to lie parallel to the interface – the directions in the plane of the interface form a degenerate set of easy axes [11] – and have no component along the normal. The in-plane nematic order, which I take to be along  $\hat{x}$ , is characterised by the two-dimensional apolar order parameter

$$\mathbf{Q} = \frac{S}{2} \begin{pmatrix} \cos 2\theta & \sin 2\theta \\ \sin 2\theta & -\cos 2\theta \end{pmatrix} \quad (\text{D1})$$

where  $\theta$  is the deviation of the local nematic order from  $\hat{x}$  and  $S$  is the magnitude of the nematic order whose steady state value is  $S_0 = \langle S \rangle$ .

The dynamics of the orientational order parameter  $\mathbf{Q}$  is coupled to the in-plane velocity field  $\mathbf{v}$ .  $\mathbf{v}$  is completely determined in terms of the particle-phase stress  $\boldsymbol{\sigma}^s$  which depends on  $\mathbf{Q}$ . The standard dynamical equation for  $\mathbf{Q}$  is

$$\dot{\mathbf{Q}} = \mathbf{Q} \cdot \boldsymbol{\Omega} - \boldsymbol{\Omega} \cdot \mathbf{Q} - \lambda \mathbf{A}^{ST} - \lambda_1 [\mathbf{Q} \cdot \mathbf{A}]^{ST} - \Gamma \mathbf{H} + \boldsymbol{\xi}^Q, \quad (\text{D2})$$

where the overdot denotes the convected derivative  $\partial_t + \mathbf{v} \cdot \nabla$ ,  $\boldsymbol{\Omega} = (1/2)[\nabla_\perp \mathbf{v} - (\nabla_\perp \mathbf{v})^T]$  is the planar vorticity tensor at the interface,  $\mathbf{A} = (1/2)[\nabla_\perp \mathbf{v} + (\nabla_\perp \mathbf{v})^T]$  is the planar strain-rate tensor at the interface, with  $|\lambda| > 1$  describing nematogens with a tendency to align under an imposed shear flow and  $|\lambda| < 1$  describing flow tumbling, the superscript  $ST$  denotes symmetrized, traceless part of a tensor,  $\mathbf{H} = [\delta F_Q / \delta \mathbf{Q}]^{ST}$  and  $\boldsymbol{\xi}^Q$  is a non-conserving noise with the correlation

$$\langle \xi_{ij}^Q(\mathbf{r}_\perp, t) \xi_{kl}^Q(\mathbf{r}'_\perp, t') \rangle = 2\Delta^Q [\delta_{ik}\delta_{jl} + \delta_{il}\delta_{jk} - \delta_{ij}\delta_{kl}] \delta(\mathbf{r}_\perp - \mathbf{r}'_\perp) \delta(t - t'). \quad (\text{D3})$$

Finally,  $\Gamma$  controls the relaxation to the equilibrium steady state, given by the free energy  $F_Q$ , in the absence of activity. The standard Landau-de Gennes free energy for a two-dimensional nematic, in a simplified one Frank constant approximation, is  $F_Q = \int d\mathbf{r}_\perp f_Q$ , with  $f_Q = (\alpha/2)(\mathbf{Q} : \mathbf{Q}) + (\beta/2)(\mathbf{Q} : \mathbf{Q})^2 + (K/2)(\nabla_\perp \mathbf{Q})^2$ , which supports an orientationally ordered phase for  $\alpha < 0$ .

Note that both in this and the PNC model, the order parameter equation is not qualitatively affected by active units entering or exiting the interfacial layer. Active units, when they enter the layer (or are assembled) do so at an *arbitrary* in-plane angle. However, this only leads to a noise in the local value of the order parameter [12, 13]. To see this heuristically, consider the following argument: the coarse-grained order parameter (here  $\mathbf{Q}$  and  $\mathbf{p}$  in the PNC model) is simply the average of the orientation of active filaments in a coarse-graining area. When a filament leaves this area (by moving into the bulk fluid or by getting disassembled) and another enters it (either directly from the bulk fluid or by being assembled from monomers, distributed in the bulk, at the interface) *at an arbitrary angle* to the ordering direction, the net effect is equivalent to the stochastic rotation of a filament within this coarse-graining area. Thus, the effect of active filament exchange with the bulk fluid is captured by a noise in (D2).

The in-plane, particle phase stress whose divergence gives the in-plane force density  $\mathbf{f}^s = \nabla_\perp \cdot \boldsymbol{\sigma}^s$  is

$$\boldsymbol{\sigma}^s = -\zeta \mathbf{Q} - \lambda \mathbf{H} - 2[\mathbf{Q} \cdot \mathbf{H}]^A - \lambda_1 [\mathbf{Q} \cdot \mathbf{H}]^{ST} - \nabla_\perp \mathbf{Q} : \frac{\partial f_Q}{\partial \nabla_\perp \mathbf{Q}}. \quad (\text{D4})$$

Here, the term with the coefficient  $\zeta$  is the active stress [6, 14] while the remaining contributions are required by Onsager symmetry to ensure that the equilibrium distribution is recovered in the limit  $\zeta = 0$ . An active stress with  $\zeta > 0$  denotes an extensile suspension, while one with  $\zeta < 0$  signifies contractility [15]. Eqs. (D2), (D4) along with the definition of the mobility (B17) (or (3) of the main text) describe the NNC model.

### 2. PNC Model: Interfacial active polar fluid composed of motile particles that diffuse in the bulk

The PNC model describes an interfacial polar phase composed of motile particles that can diffuse in the bulk fluid as can be realised in a system of elongated, active Brownian particles [16] at the boundary of a bulk fluid or at a

two-fluid interface. It shares similarities with the NNC model. As in the NNC model, the interfacial concentration field  $c$  is non-hydrodynamic in this model for precisely the same reason. Therefore, to describe the motile phase in the PNC model, I need to specify the dynamics of a polar order parameter  $\mathbf{p}$  which couples to the in-plane velocity field. The polar order parameter is taken to be disposed, on average, along  $\hat{x}$ :  $\mathbf{p} = p(\cos\theta, \sin\theta)$  where  $p$  is the magnitude of the polar order and  $\theta$  denotes the local deviation of the polarisation from  $\hat{x}$ . The in-plane velocity field is determined by a  $\mathbf{p}$ -dependent stress  $\boldsymbol{\sigma}^s$  and the mobility (B17). The dynamics of  $\mathbf{p}$  is described by

$$\dot{\mathbf{p}} + v_p \mathbf{p} \cdot \nabla \mathbf{p} + \boldsymbol{\Omega} \cdot \mathbf{p} = -\lambda \mathbf{p} \cdot \mathbf{A} - \lambda_p \nabla_{\perp}^2 \mathbf{v} - \Gamma_p \mathbf{h} + \boldsymbol{\xi}^p \quad (\text{D5})$$

where  $v_p$  denotes active self-advection due to the motility of the polar particles,  $F_p = \int d\mathbf{r}_{\perp} [(\alpha/2)\mathbf{p}^2 + (\beta/4)\mathbf{p}^4 + (K/2)(\nabla_{\perp} \mathbf{p}^2) + K_p \mathbf{p}^2 \nabla_{\perp} \cdot \mathbf{p}] = \int d\mathbf{r}_{\perp} f_p$  is the standard free energy for polar liquid crystals,  $\mathbf{h} = \delta F_p / \delta \mathbf{p}$  and the noise  $\boldsymbol{\xi}^p$  has the correlation  $\langle \xi_i^p(\mathbf{r}_{\perp}, t) \xi_j^p(\mathbf{r}'_{\perp}, t') \rangle = 2\Delta^p \delta_{ij} \delta(\mathbf{r}_{\perp} - \mathbf{r}'_{\perp}) \delta(t - t')$ . There are additional, permitted active terms in the polarisation equation at the same order in gradients and fields of the form  $\mathbf{p} \nabla \cdot \mathbf{p}$  and  $\nabla \mathbf{p}^2$  [14, 17–19]. However, these do not ultimately affect the hydrodynamic fluctuations of the polar phase [19] because they do not appear in the equation for angular fluctuations. Therefore, I disregard them. The particle phase stress tensor for a polar state is [20, 21]

$$\boldsymbol{\sigma}^s = -\zeta \left( \mathbf{p} \mathbf{p} - \frac{p^2}{2} \mathbf{I} \right) + \zeta_p [\nabla_{\perp} \mathbf{p} + (\nabla_{\perp} \mathbf{p})^T] - 2\lambda [\mathbf{p} \mathbf{h}]^S + \lambda_p [\nabla_{\perp} \mathbf{p}]^S - 2[\mathbf{p} \mathbf{h}]^A - \nabla_{\perp} \mathbf{p} \cdot \frac{\partial f_p}{\partial (\nabla_{\perp} \mathbf{p})} \quad (\text{D6})$$

where the superscripts  $S$  and  $A$  describe symmetric and antisymmetric parts of a tensor respectively and the final term is Ericksen stress [22]. The in-plane divergence of this stress is the surface force for the PNC model  $\mathbf{f}^s = \nabla_{\perp} \cdot \boldsymbol{\sigma}^s$ . Eqs. (D5) and (D6) together with the definition of mobility completely specify the PNC model.

### 3. NC Model: Interfacial active nematic composed of nematogenic species living at the interface

In this case, the concentration  $c$  of active particles at the interface is conserved. The NC model describes an interfacial active nematic in which the concentration of the active particles  $c$  at the interface is conserved. As a consequence,  $c$  is an additional hydrodynamic variable that couples with the in-plane order parameter and the velocity both in this and the PC models. The effective free energy (with a coupling between  $c$  and  $\mathbf{Q}$ ) is  $F_{Qc} = F_Q + \int d\mathbf{r}_{\perp} [g(c) + A_{Qc} \mathbf{Q} : \nabla_{\perp} \nabla_{\perp} c + A_{Qc2} \mathbf{Q} : \nabla_{\perp} c \nabla_{\perp} c]$  where  $g(c)$  is a function of concentration. The dynamics of the  $\mathbf{Q}$  tensor has the same form as in the NNC model (see (D2)):

$$\dot{\mathbf{Q}} = \mathbf{Q} \cdot \boldsymbol{\Omega} - \boldsymbol{\Omega} \cdot \mathbf{Q} - \lambda \mathbf{A}^{ST} - \lambda_1 [\mathbf{Q} \cdot \mathbf{A}]^{ST} - \Gamma \mathbf{H} + \boldsymbol{\xi}^Q, \quad (\text{D7})$$

with  $\mathbf{H} = [\delta F_{Qc} / \delta \mathbf{Q}]^{ST}$ . While the coefficients such as  $\lambda$  now, in principle, depend on the concentration  $c$ , this turns out to not affect the linear (in)stability of the ordered state ( $\lambda(c) \equiv \lambda(c_0) + \lambda'(c_0)\delta c + \dots$  where the prime denotes differentiation with respect to  $c$  and  $\delta c$  is the deviation of  $c$  about a steady state value  $c_0$ ). The part of  $\lambda$  depending on the fluctuations of the concentration about its steady-state value – to the lowest order in  $\delta c$ ,  $\lambda'(c_0)\delta c$  – only contributes nonlinear terms to the equation of motion). The concentration dynamics has the form

$$\partial_t c = -\nabla_{\perp} \cdot (c \mathbf{v}) + \Gamma_c \nabla_{\perp}^2 \frac{\delta F_{Qc}}{\delta c} + \nabla_{\perp} \cdot \mathbf{J}^a + \xi_c \quad (\text{D8})$$

where  $\mathbf{J}^a = \zeta_c \nabla_{\perp} [g_{Q1}(c) \nabla_{\perp} \cdot \{g_{Q2}(c) \mathbf{Q}\}]$  for an apolar system, with  $g_{Q1}(c)$  and  $g_{Q2}(c)$  being arbitrary functions of the concentration field, and the conserving, spatiotemporally white noise  $\xi_c$  has the correlation  $\langle \xi_c(\mathbf{r}_{\perp}, t) \xi_c(\mathbf{r}'_{\perp}, t') \rangle = -2\Delta^c \nabla_{\perp}^2 \delta(\mathbf{r}_{\perp} - \mathbf{r}'_{\perp}) \delta(t - t')$ . The second term in (D8) controls the relaxation to equilibrium in the absence of activity while the final term is the active curvature current [14, 23, 24]. Finally, the particle phase stress tensor

$$\boldsymbol{\sigma}^s = -\Pi(c) \mathbf{I} - \zeta(c) \mathbf{Q} - \lambda \mathbf{H} - 2[\mathbf{Q} \cdot \mathbf{H}]^A - \lambda_1 [\mathbf{Q} \cdot \mathbf{H}]^{ST} - \nabla_{\perp} \mathbf{Q} : \frac{\partial f_Q}{\partial \nabla_{\perp} \mathbf{Q}}. \quad (\text{D9})$$

is also modified from (D4): the active stress coefficient  $\zeta$  generically depends on the concentration  $-\zeta(c) \mathbf{Q}$ . More generally, all coefficients now depend on  $c$ , but the concentration-dependence of the other coefficients do not affect the linear stability of the interfacial ordered state. There is also an additional isotropic pressure-like term  $-\Pi_c(c) \mathbf{I}$ , where  $\mathbf{I}$  is the rank two identity tensor which, in general, has both active and passive contributions. Further active nonlinear terms of the form  $\nabla_{\perp} c \nabla_{\perp} c$  [3–5] are also allowed in the stress, but they do not affect the stability of a homogeneous ordered phase.

#### 4. PC Model: Interfacial active polar fluid composed of polar species living at the interface

The PC model describes a floating flock of purely interface or boundary-associated motile units. The polarisation dynamics of the flocks is the same as in the PNC model (see Eq. (D5))

$$\dot{\mathbf{p}} + v_p \mathbf{p} \cdot \nabla \mathbf{p} + \boldsymbol{\Omega} \cdot \mathbf{p} = -\lambda \mathbf{p} \cdot \mathbf{A} - \lambda_p \nabla_{\perp}^2 \mathbf{v} - \Gamma_p \mathbf{h} + \boldsymbol{\xi}^p, \quad (\text{D10})$$

with a modified definition of  $\mathbf{h} = \delta F_{pc} / \delta \mathbf{p}$  where  $F_{pc} = F_p + \int d\mathbf{r}_{\perp} [g(c) + \gamma \mathbf{p} \cdot \nabla_{\perp} c]$  with  $g(c)$  being an arbitrary function of the concentration field and the final term is the spontaneous splay energy familiar in studies of polar liquid crystals [25]. The coefficients such as  $\lambda$  and  $\lambda_p$  can now depend on the concentration field  $c$ , but this will not affect the stability of a homogeneous polar state. The dynamics of the concentration field is again described by (D8)

$$\partial_t c = -\nabla_{\perp} \cdot (c \mathbf{v}) + \Gamma_c \nabla_{\perp}^2 \frac{\delta F_{Qc}}{\delta c} + \nabla_{\perp} \cdot \mathbf{J}^a + \xi_c \quad (\text{D11})$$

with, however, a distinct active current  $\mathbf{J}^a = v_c(c) \mathbf{p}$  proportional to the polarisation itself. This models the active motility of the flocks. Finally, as in the NC model, the particle phase stress tensor is modified from (D6) due to the concentration dependence of the active stresses  $\zeta(c) (\mathbf{p}\mathbf{p} - p^2 \mathbf{I}/2) + \zeta_p(c) [\nabla_{\perp} \mathbf{p} + (\nabla_{\perp} \mathbf{p})^T]$  and the presence of a surface pressure-like isotropic stress  $-\Pi_c(c) \mathbf{I}$ . Further, all phenomenological coefficients now, in principle, depend on the concentration field. That is,

$$\boldsymbol{\sigma}^s = -\Pi(c) \mathbf{I} - \zeta(c) \left( \mathbf{p}\mathbf{p} - \frac{p^2 \mathbf{I}}{2} \right) + \zeta_p(c) [\nabla_{\perp} \mathbf{p} + (\nabla_{\perp} \mathbf{p})^T] - 2\lambda [\mathbf{p}\mathbf{h}]^S + \lambda_p [\nabla_{\perp} \mathbf{p}]^S - 2[\mathbf{p}\mathbf{h}]^A - \nabla_{\perp} \mathbf{p} \cdot \frac{\partial f_p}{\partial (\nabla_{\perp} \mathbf{p})} \quad (\text{D12})$$

#### Appendix E: Detailed demonstration that interfacial order is long-ranged

In this supplementary section, I will expand on the discussion of the stability of the interfacial nematic flock in the NNC model and discuss its long-range nature (which is best demonstrated by calculating the exact roughness exponent). To demonstrate the stability of nematic phase in the NNC model, I expand Eqs. (D2), and (D4) of the NNC model with (B17) to linear order in fluctuations about a perfectly ordered phase which, without loss of generality, I take to have the value  $S_0 = 1$  (i.e., take  $S_0$  to have its maximum possible value when  $\alpha$  is negative and assumes its minimum value, which I take to be  $-\beta$ ). Writing  $S = 1 + \delta S$ , the equation of motion for  $\delta S$  from (D2), to the lowest order in gradients is simply  $\partial_t \delta S = -2\Gamma |\alpha| \delta S$ . This implies that the fluctuations of the order parameter magnitude relax within a finite time  $\sim (\Gamma \alpha)^{-1}$  and, therefore do not affect the long-time, large-scale behaviour of the ordered phase. The angle field, in contrast, is a Goldstone mode corresponding to broken rotation symmetry and is, therefore, hydrodynamic. For a state oriented along  $\hat{x}$ , the linearised angular dynamics from (D2) is

$$\partial_t \theta = \Omega_{xy} - \lambda A_{xy} + \Gamma_{\theta} K \nabla_{\perp}^2 \theta + \xi, \quad (\text{E1})$$

where  $\Gamma_{\theta} = \Gamma/4$  and  $\langle \xi(\mathbf{r}_{\perp}, t) \xi(\mathbf{r}'_{\perp}, t') \rangle = 2\Delta \delta(\mathbf{r}_{\perp} - \mathbf{r}'_{\perp}) \delta(t - t') \delta(z)$ , with  $\Delta = \Delta^Q/4$ . Similarly, expanding the interfacial particle-phase force density  $\mathbf{f}^s = i \mathbf{q}_{\perp} \cdot \boldsymbol{\sigma}^s$  (D4), to the lowest order in wavenumbers, I obtain  $\mathbf{f}^s = -i\zeta(q_y \theta \hat{x} + q_x \theta \hat{y})$ . Combining this with the lowest order in wavenumber  $\sim q^{-1}$  part of the mobility (B17) yields the in-plane velocity field and the relaxation rate of the angular fluctuations to leading order in wavenumbers:

$$\partial_t \theta = -\frac{\zeta}{4\eta} \frac{q_x^4(\lambda - 1) + q_y^4(\lambda + 1)}{|q_{\perp}|^3} \theta + \mathcal{O}(q_{\perp}^2) + \xi = \frac{\zeta |q_{\perp}|}{4\eta} \left[ \cos(2\phi) [1 - \lambda \cos(2\phi)] - \frac{\lambda}{2} \sin^2(2\phi) \right] \theta + \mathcal{O}(q_{\perp}^2) + \xi, \quad (\text{E2})$$

where in the second equality,  $\phi$  is the angle between  $\mathbf{q}_{\perp}$  and the mean ordering direction  $\hat{x}$ . This is the angular dynamics described in the main text. Eq. (E2) implies that the relaxation rate for angular fluctuations is *positive* for all  $\phi$  when  $|\lambda| > 1$  – i.e., flow-aligning – and  $\zeta \lambda > 0$ . To see this, first consider  $\zeta > 0$  and  $\lambda > 1$ . Then, for the relaxation rate to be positive, the term within the square brackets has to be  $< 0$  for all  $\phi$  i.e., all of its extreme values must be negative. The extreme values of this term, which can be expressed as  $[\cos 2\phi - (\lambda/2)(1 + \cos^2 2\phi)]$  are at  $\phi = (2n + 1)\pi/2, n\pi$  or at  $\cos 2\phi = 1/\lambda$  and all of them are negative for  $\zeta > 0$  and  $\lambda > 1$ :  $[\cos 2\phi - (\lambda/2)(1 + \cos^2 2\phi)]|_{\phi=n\pi} = [1 - \lambda] < 0$ ,  $[\cos 2\phi - (\lambda/2)(1 + \cos^2 2\phi)]|_{\phi=(2n+1)\pi/2} = [-1 - \lambda] < 0$  and  $[\cos 2\phi - (\lambda/2)(1 + \cos^2 2\phi)]|_{\cos \phi=1/\lambda} = [(1/\lambda) - (\lambda/2)\{1 + (1/\lambda)^2\}] = 1/(2\lambda) - \lambda/2 < 0$ . A similar argument shows that the relaxation rate is positive, i.e., the planar ordered phase is stable, when  $\zeta < 0$  and  $\lambda < -1$ . This directly demonstrates that, contrary to popular belief, a two-dimensional planar nematic phase is realised in the fully momentum-conserved NNC model.



In contrast, the nematic phase is unstable to fluctuations in flow-tumbling systems  $|\lambda| < 1$  for either sign of activity – extensile systems ( $\zeta > 0$ ) are unstable for  $\phi \approx 0$ , i.e., bend, and contractile systems ( $\zeta < 0$ ) are unstable for splay,  $\phi \approx \pi/2$  – or even in flow-aligning systems when  $\zeta\lambda < 0$ .

When the nematic state is linearly destabilised in the NNC model, a patterned state is expected to appear [26–28] whose wavenumber, which is expected to coincide with the fastest growing mode, is  $q_\perp^c = \text{Max}[\zeta\{2\cos 2\phi - \lambda(1 + \cos^2 2\phi)\}/(8\eta\Gamma_\theta K_r(\phi))]$ , where Max denotes the maximum value of a function and  $\Gamma_\theta K_r(\phi)$  denotes the coefficient of the  $\mathcal{O}(q_\perp^2)$  term in (E2), with  $K_r(\phi)$  being the effective activity-renormalised Frank elasticity, which in passive systems would have been just  $-\Gamma_\theta K$  but here will have active corrections as displayed in the supplementary section I. Note that  $K_r$  explicitly depends on the Saffmann-Delbrück length and, hence, the scale of the patterns beyond the instability depends on this length.

Concentrating on the stable nematic phase in the NNC model, Eq. (E2) implies that the relaxation rate of angular fluctuations scales as  $|q_\perp|$  along *all* directions of the wavevector space unlike the relaxation rate of passive nematics or active nematics on substrates both of which scale as  $\sim q_\perp^2$  [14, 23, 24]. This is due to a combination of activity and momentum-conserved fluid dynamics-induced long-range interactions. While the interaction is not long-enough ranged (i.e., it decays too fast) to make the orientational Goldstone mode massive [20, 29], which remains hydrodynamic  $\omega \propto -i|q_\perp|$ , it drastically reduces the director fluctuations. From Eq. (E2), the static structure factor of angular fluctuations

$$\langle |\theta(\mathbf{q}_\perp, t)|^2 \rangle = \frac{8\eta\Delta}{\zeta|q_\perp|[\lambda\{1 + \cos^2(2\phi)\} - 2\cos(2\phi)]}. \quad (\text{E3})$$

This diverges as  $\sim 1/|q_\perp|$  along *all* directions of the wavevector space – more slowly than in two-dimensional rotation symmetry broken states with short-range interactions, where the divergence as  $\sim 1/q_\perp^2$  leads to the destruction of LRO [30]. The depression of the order parameter from its perfectly ordered value  $S_0 = 1$  due to fluctuations is obtained using  $\langle S \rangle/S_0 = \langle \cos 2\theta \rangle \equiv e^{-W}$  where  $W = 2\langle \theta(\mathbf{r}_\perp, t)^2 \rangle = 2 \int (d^2 q_\perp / 4\pi^2) \langle |\theta(\mathbf{q}_\perp, t)|^2 \rangle$  evaluates to

$$W = 2 \int d|q_\perp| \int \frac{2\eta\Delta d\phi}{\pi^2 \zeta [\lambda\{1 + \cos^2(2\phi)\} - 2\cos(2\phi)]} \propto \Lambda\Delta, \quad (\text{E4})$$

with  $\Lambda$  being a wavenumber cut-off. Since  $W$  is finite,  $\langle S \rangle$  does not generically vanish due to fluctuations even in infinite systems, unlike in, for instance, X-Y model [30], implying that at least for small enough  $\Delta$ , a long-range ordered nematic phase exists. More formally, the Debye-Waller factor  $e^{-2W}$  is nonzero even for infinite systems implying long-range order.

This discussion of the existence of long-range interfacial nematic order in the NNC model considered only linear fluctuations. I now demonstrate that it remains qualitatively correct even taking nonlinearities into account by using the standard renormalisation group logic. For this, I rescale lengths, time and the angle field as  $x \rightarrow bx$ ,  $y \rightarrow b^\mu y$ ,  $t \rightarrow b^z t$  and  $\theta \rightarrow b^\chi \theta$ , where  $\mu$  is the anisotropy exponent,  $z$  is the dynamical exponent and  $\chi$  is the roughness exponent. Within the linear theory, these exponents can be determined from the knowledge of the static (E3) and dynamic structure factors

$$\langle |\theta(\mathbf{q}_\perp, \omega)|^2 \rangle = \frac{128\eta^2\Delta}{(8\eta\omega)^2 + [\zeta|q_\perp|\{\lambda(1 + \cos^2 2\phi) - 2\cos 2\phi\}]^2}. \quad (\text{E5})$$

From (E3)  $\langle \theta(0, t)\theta(\mathbf{r}_\perp, t) \rangle = \int (d\mathbf{q}_\perp / 4\pi^2) e^{i\mathbf{q}_\perp \cdot \mathbf{r}_\perp} \langle |\theta(\mathbf{q}_\perp, t)|^2 \rangle \sim 1/|\mathbf{r}_\perp|$ , which implies  $\chi = -1/2$ . Furthermore, since Eq. (E3) scales the same way along *all* directions of the wavevector space, the anisotropy exponent  $\mu = 1$ . Finally, balancing  $\omega$  against the damping term in (E5) yields  $\omega \propto q_\perp$  and, therefore, the dynamical exponent  $z = 1$  within the linearised theory. The values of these linear exponents may also be obtained more formally by demanding that the size of fluctuations of  $\theta$  remain fixed upon rescaling i.e., by ensuring that the relaxation rate and the noise strength  $\Delta$  remain unchanged. Since the relaxation rate must remain unchanged along all directions of wavevector space,  $\mu = 1$ . Since the relaxation rate  $\sim |q_\perp|$ ,  $z = 1$  as well. Under rescaling, the noise strength scales as  $\Delta \rightarrow \Delta b^{z-\mu-1-2\chi}$  implying that for it to remain unchanged,  $\chi = -1/2$  since  $z = \mu = 1$ . Unsurprisingly, both arguments yield the same values for the linear exponents. With these *linear* exponents, I now assess the importance of possible nonlinear terms in (E2) by simply checking whether the coefficients of these grow or decay under rescaling. The most relevant nonlinearities that can appear in (E2) are terms that have one power of the velocity field  $\mathbf{v}$  and one power of  $\theta$ , along with a gradient operator, such as the one due to advection  $\mathbf{v} \cdot \nabla_\perp \theta$ . This scales as  $q_\perp(\theta^2)_q$  since  $\mathbf{v} \sim \Phi(\phi)\theta$  where  $\Phi(\phi)$  is a vector function that depends on  $\phi$ , but not on  $|q_\perp|$ . The most relevant nonlinearity not involving the velocity field contains two powers of the gradient and is quadratic in  $\theta$  [31–33] and is, therefore, subdominant to this. The coefficient of the most dominant nonlinearity  $q_\perp(\theta^2)_q$  scales under rescaling as  $b^{z-1+\chi} = b^\chi$ . Since within the linear theory,  $\chi = -1/2 < 0$ , this clearly decays under rescaling and, therefore, is irrelevant. This implies that this model

has *no* relevant nonlinearity and the linear theory is *exact* i.e., (E2), (E3) and (E5) describe the exact long-distance, large-time properties of a boundary-associated active nematic phase in a momentum-conserved system. In particular, the low-noise, long-range ordered nematic state predicted on the basis of the linear theory, survives even upon taking nonlinearities into account.

### Appendix F: Stability of a nematic film floating in a confined channel

The calculations presented in the main text assumed orientational order at interfaces between bulk fluids. However, most experimental chambers, for instance, the one in [34] or the one in [35] are strongly confined in one direction. In this supplementary section, I show that a floating film [34] or a two-fluid interface [35] supports active uniaxial order even in this geometry. For simplicity, I again consider viscosity-matched fluids above and below the interface or the film, with viscosity  $\eta$ . This can be easily generalised to fluids with two different viscosities, without any qualitative modification of the results, by simply replacing the viscosity with  $(\eta_b + \eta_t)/2$ . I consider a film floating at  $z = 0$  in a channel extending from  $z = -H$  to  $z = H$  i.e., of height  $2H$  along the  $z$  direction. The constitutive equation for the three-dimensional velocity field is

$$\eta \nabla^2 \mathbf{V} = \nabla \Pi + \zeta (\partial_y \theta \hat{x} + \partial_x \theta \hat{y}) \delta(z) \quad (\text{F1})$$

while the dynamics of  $\theta$  is still described by (E1). The channel geometry is effectively taken into account by taking  $\mathbf{V} = 0$  for  $-2\pi/H < q_z < 2\pi/H$ . Therefore, the integral over  $q_z$  to obtain  $v_x$  and  $v_y$  is not from  $\{-\infty, \infty\}$  but from  $\{-\infty, -2\pi/H\} \cup \{2\pi/H, \infty\}$ . This yields

$$v_x = \int_{-\infty}^{\infty} \frac{dq_z}{2\pi} \frac{-f_y^s q_x q_y + f_x^s (q_y^2 + q_z^2)}{\eta q^4} - \int_{-2\pi/H}^{2\pi/H} \frac{dq_z}{2\pi} \frac{-f_y^s q_x q_y + f_x^s (q_y^2 + q_z^2)}{\eta q^4} = \frac{-f_y^s q_x q_y + f_x^s (q_x^2 + 2q_y^2)}{4\eta |q_{\perp}|^3} + \frac{H q_y \mathbf{f}^s \cdot \mathbf{q}_{\perp}}{\eta q_{\perp}^2 (4\pi^2 + H^2 q_{\perp}^2)} - \tan^{-1} \left( \frac{2\pi}{H |q_{\perp}|} \right) \frac{-f_y^s q_x q_y + f_x^s (q_x^2 + 2q_y^2)}{2\eta \pi |q_{\perp}|^3} \quad (\text{F2})$$

$$v_y = \int_{-\infty}^{\infty} \frac{dq_z}{2\pi} \frac{-f_x^s q_x q_y + f_y^s (q_y^2 + q_z^2)}{\eta q^4} - \int_{-2\pi/H}^{2\pi/H} \frac{dq_z}{2\pi} \frac{-f_x^s q_x q_y + f_y^s (q_y^2 + q_z^2)}{\eta q^4} = \frac{-f_x^s q_x q_y + f_y^s (q_x^2 + 2q_y^2)}{4\eta |q_{\perp}|^3} + \frac{H q_x \mathbf{f}^s \cdot \mathbf{q}_{\perp}}{\eta q_{\perp}^2 (4\pi^2 + H^2 q_{\perp}^2)} - \tan^{-1} \left( \frac{2\pi}{H |q_{\perp}|} \right) \frac{-f_x^s q_x q_y + f_y^s (q_x^2 + 2q_y^2)}{2\eta \pi |q_{\perp}|^3} \quad (\text{F3})$$

where  $f_x^s = -i\zeta q_y \theta$  and  $f_y^s = -i\zeta q_x \theta$ . Using these values for  $\mathbf{v}$  in (E1), I recover (E2) for  $H \gg 1/|q_{\perp}|$ , i.e., when the in-plane scales are much smaller than the confinement scale, as expected. Interestingly, for  $H \ll 1/|q_{\perp}|$  i.e., for in-plane scales much larger than the confinement height, the angular dynamics becomes

$$\partial_t \theta = \left[ \frac{H q_{\perp}^2 \zeta}{4\pi^2 \eta} (\cos 2\phi - \lambda) - K q_{\perp}^2 \right] \theta, \quad (\text{F4})$$

where  $\phi$  is the angle between the ordering direction,  $\hat{x}$ , and  $\mathbf{q}_{\perp}$ . The first term is *stabilising* when  $\lambda \zeta > 0$  and  $|\lambda| > 1$  which is exactly the condition for stability of the orientational order in an unbounded fluid. Therefore, orientational order in a film floating in a channel [34] or at a two-fluid interface in a channel can remain stable even at arbitrarily high active drive. However, due to the long-range fluid interactions being cut-off by the confinement at the scale  $H$ , the relaxation rate of angular fluctuations now scales as  $\sim q_{\perp}^2$  for  $|q_{\perp}| \ll 1/H$  instead of as  $|q_{\perp}|$  as it would in an unbounded system. This implies that the stable nematic phase in a film or at a two-fluid interface in a channel is only quasi-long-range ordered instead of being truly long-ranged.

### Appendix G: Defect interactions in the nematic phase of NNC model

The discussions of stability and long-range order of interfacial active nematics, up to this point, considered only smooth director fluctuations about an ordered state and ignored topological defects. Yet, in bulk active nematics, dynamics of topological defects are known to drive the eventual spatiotemporally chaotic state [7, 36, 37]. Indeed,  $+1/2$  defects in nematics are geometrically polar [22, 30, 38] and, therefore, are rendered motile by activity [39–43]. Since  $-1/2$  defects have a three-fold symmetry,  $\pm 1/2$  defect pairs in active nematics generically unbind at low noise

strengths [39]. While a full examination of defect dynamics in the interfacial nematic phase, including their advection by active flows leading to non-reciprocal defect interactions [44, 45], is beyond the scope of this article, I now argue that the long-range interaction that stabilises the ordered phase to director fluctuations also makes the unbinding of  $\pm 1/2$  defects much less likely than in other active nematic systems, both wet and dry.

The modification of the *attractive* interaction between  $\pm 1/2$  defect pairs due to the combination of fluid flow and activity can be understood via an analogy with the passive two-dimensional  $X - Y$  model with dipolar interactions [46–48]. This analogy is not perfect: the dipolar interaction has the free energy density  $F_{\text{dip}} = \int_{\mathbf{r}_\perp} \int_{\mathbf{r}'_\perp} \partial_\alpha \theta(\mathbf{r}_\perp) \partial'_\beta \theta(\mathbf{r}'_\perp) / |\mathbf{r}_\perp - \mathbf{r}'_\perp|$ . Therefore, the relaxation rate for the spin fluctuations in two-dimensional dipolar  $X - Y$  model vanishes at small wavenumbers as  $\sim q_\perp$  for *most* directions of the wavevector space. Unlike the interfacial active nematics, however, the dispersion relation is  $\omega \sim -iq_y^2/|q_\perp|$  and, therefore, vanishes as  $q_x^2$  for fluctuations along the ordering direction [20, 48, 49]. This implies that the two models belong to distinct universality classes with the dynamical exponent  $z = 2$ , the anisotropy exponent  $\mu = 3/2$  and the roughness exponent  $\chi = -1/4$  for the dipolar  $X - Y$  model. The higher value of  $\chi$  in the dipolar  $X - Y$  model compared to interfacial active nematics demonstrates that it has a lower degree of order, as expected, since the relaxation rate of fluctuations in the latter scale as  $|q_\perp|$  in *all* directions of the wavevector space. Nevertheless, the imperfect analogy between the two models proves fruitful in understanding defect interactions in interfacial active nematics. The linear dynamics of the interfacial active nematic (E2) can be derived from an effective free energy

$$F_{\text{eff}}[\theta] = \frac{1}{2} \int d|q_\perp| \int d\phi \left[ \frac{|\zeta|C(\phi)}{4\Gamma_\theta\eta} \frac{1}{|q_\perp|} + K_r \right] q_\perp^2 |\theta|^2, \quad (\text{G1})$$

where  $C(\phi) = \cos(2\phi)[1 - \lambda \cos(2\phi)] - (\lambda/2) \sin^2(2\phi)$ . Importantly, the first term in the square bracket has the same spatial character as the dipolar energy in a two-dimensional  $X - Y$  model with dipolar interactions [46–48], but as advertised, a different angular character, with  $C(\phi)$  being strictly positive in the stable phase being considered here (in dipolar magnets, the corresponding  $C(\phi)$  vanishes as  $\phi = 0$ ). Ignoring, for the moment, the motility of  $+1/2$  defects, I use an argument presented in [47] for vortex interactions in the passive dipolar  $X - Y$  model to obtain the defect interactions in the NNC model. The singular part of the angle field due to a defect at the origin with charge  $s$  is  $\bar{\theta}(|r_\perp|, \phi') = 2\pi s \int_{|q_\perp|, \phi} e^{i|q_\perp||r_\perp| \cos(\phi - \phi')} / q_\perp^2$ . From this, following [47] the defect interaction energy between two defects (which can be easily generalised to an arbitrary number of defects), with charges  $s_1$  and  $s_2$  and at positions 0 and  $|r_\perp|(\cos \phi', \sin \phi')$  is

$$F_{\text{def}} = \pi^2 s_1 s_2 \int_{q_\perp, \phi} e^{-i|q_\perp||r_\perp| \cos(\phi - \phi')} \left[ \frac{K_r}{q_\perp^2} + \frac{|\zeta|C(\phi)}{4\Gamma_\theta\eta} \frac{1}{|q_\perp|} \right]. \quad (\text{G2})$$

As is well-known, the infrared divergences cancel for a charge-neutral system finally yielding a defect interaction energy (for one of the defects at the origin) which, when written in real space, has the form

$$F_{\text{int}} = -s_1 s_2 \left[ \frac{\pi K_r}{2} \ln \left( \frac{|r_\perp|}{a} \right) + \frac{\zeta}{\Gamma_\theta\eta} \alpha |r_\perp| \right] \quad (\text{G3})$$

where  $a$  is the size of the defect core and  $\alpha > 0$  is a positive constant whose determination requires a detailed calculation beyond the scope of this heuristic argument. The interaction energy scaling as  $|r_\perp|$  is stronger than the usual logarithmic potential that binds defects in passive systems with short-range interactions and is equivalent to the potential between vortices in dipolar  $X - Y$  models. In effect, here activity effectively leads to an additional elasticity which *diverges* as  $1/|q_\perp|$  as  $q_\perp \rightarrow 0$  or as  $r_\perp$  as  $r_\perp \rightarrow \infty$  leading to the extra contribution. In passive dipolar  $X - Y$  models an interaction energy of the form (G3) immediately implies that defects are bound in the low-temperature ordered phase. The situation is more complicated here because of two aspects of defect dynamics in active systems which I disregarded. First of these is the self-propulsion of  $+1/2$  defects. Within a one-dimensional approximation, this leads to an effective *repulsive* potential between oppositely charged defects that scales as  $|r_\perp|$  and should compete against the attractive potential  $\propto \zeta$ . This repulsive interaction also depends linearly on  $\zeta$  with the full effective potential becoming  $F_{\pm 1/2} = F_{\text{int}}|_{s_1 s_2 = -1/4} - |v||r_\perp|$  where  $|v| \propto \zeta$  is the motility of the  $+1/2$  defect [39, 42]. Therefore, understanding whether  $\pm 1/2$  defect pairs remain bound at low noise strengths in interfacial active nematics requires a detailed calculation of the coefficients of the defect motility and attractive interaction. However, [39] demonstrates that at intermediate noise strengths fluctuations isotropise the direction of motion of the  $+1/2$  defects making them diffusive and weakening the effect of motility such that it simply renormalises the effective Frank elasticity. While that calculation ignores all effects of fluid flow, a similar argument should hold in this case as well implying that at least at intermediate noise strengths, the defects should remain strongly bound making the long-range ordered phase described here possible. The second aspect of defect dynamics disregarded here is the non-reciprocal interaction between active defects [44, 45, 50]. A consideration of these complexities will be discussed elsewhere. Notwithstanding these caveats, this heuristic discussion suggests that the long-range ordered nematic state discussed here should be observable in experiments and will not be inevitably destroyed due to the unbinding of defects.

## Appendix H: Polar phase in the PNC model

In this supplementary section, I examine the polar phase of the PNC model. Expanding (D5) and (D6) with the mobility (B17) in angular fluctuations  $\mathbf{p} = p_0(\cos\theta, \sin\theta)$  to leading order in wavenumber, about a perfectly ordered state with  $p_0 = 1$ , I obtain the angular dynamics

$$\partial_t \theta = \frac{\zeta|q_\perp|}{4\eta} \left[ \cos(2\phi)[1 - \lambda \cos(2\phi)] - \frac{\lambda}{2} \sin^2(2\phi) \right] \theta - i v_p (|q_\perp| \cos \phi) \theta - \Gamma_p K_r^p q_\perp^2 \theta + \xi, \quad (\text{H1})$$

where  $K_r^p$  is the effective Frank elasticity renormalised by activity displayed in supplementary section I and  $\langle \xi(\mathbf{r}_\perp, t) \xi(\mathbf{r}'_\perp, t') \rangle = 2\Delta^p \delta(\mathbf{r}_\perp - \mathbf{r}'_\perp) \delta(t - t') \delta(z)$ . The only qualitative difference between this and (E2) is the propagating part  $\propto v_p$  which is due to the motility of the polar particles. However, this doesn't affect the conditions for the stability of the polar phase which are equivalent to the ones discussed for the nematic phase in the NNC model: the interfacial polar phase is stable when  $|\lambda| > 1$  and  $\zeta\lambda > 0$ . Further, the static structure factor of angular fluctuations has the same form as (E3) implying that the polar order is long-ranged. The argument presented for the irrelevance of all nonlinearities in the NNC model also remains valid in the PNC model, implying that the exact exponents for the polar phase are  $z = \mu = 1$  and  $\chi = -1/2$ . Thus, just as its nematic counterpart, a motile polar phase is stable and displays long-range order at the boundary of a bulk fluid even though bulk polar ordering is forbidden.

While the focus of this article is on investigating the properties and the possibility of a spontaneous rotation symmetry-broken interfacial state, I now briefly examine the properties of the order-disorder transition *to* that state. That is, I now examine a state in which  $p_0 \neq 1$  but  $p_0 \rightarrow 0^+$  and  $\alpha \rightarrow 0^-$ . In this case, the *full* polarisation vector is a *slow* variable. Therefore, I now expand  $\mathbf{p} = (p_0 + \delta p)(\cos\theta, \sin\theta)$  with a  $p_0 = \sqrt{|\alpha|/\beta}$  and write the coupled equation for  $\delta p$  and  $\theta$  using (D5) and (D6). This yields

$$\partial_t \delta p = -2\Gamma_p |\alpha| \delta p - i v_p p_0 |q_\perp| \cos \phi \delta p - \frac{p_0^2 \lambda |q_\perp| (\zeta + 2|\alpha|\lambda)}{16\eta} (3 - \cos 4\phi) \delta p + \frac{p_0^3 \lambda \zeta |q_\perp| \sin 4\phi}{16\eta} \theta, \quad (\text{H2})$$

$$\partial_t \theta = -\frac{p_0 |q_\perp| (\zeta + 2|\alpha|\lambda) (\lambda \cos 2\phi - 2)}{8\eta} \delta p - i v_p p_0 |q_\perp| \cos \phi \theta - \frac{p_0^2 |q_\perp| \zeta [\lambda(3 + \cos 4\phi) - 4 \cos 2\phi]}{16\eta} \theta. \quad (\text{H3})$$

This implies the eigenfrequencies

$$\omega_p = p_0 v_p |q_\perp| \cos \phi - 2i|\alpha|\Gamma_p - i \frac{p_0^2 \lambda (\zeta + 2|\alpha|\lambda) (3 - \cos 4\phi)}{16\eta} |q_\perp| \quad (\text{H4})$$

and

$$\omega_\theta = p_0 v_p |q_\perp| \cos \phi - i \frac{p_0^2 \zeta [\lambda(3 + \cos 4\phi) - 4 \cos 2\phi]}{16\eta} |q_\perp|. \quad (\text{H5})$$

While it may seem the  $\mathcal{O}(q_\perp)$  relaxational terms vanish in the limit  $p_0 \rightarrow 0^+$ , that is not the case. It is known for equilibrium liquid crystals [51, 52], the flow-alignment parameter  $\lambda$  itself diverges at (and above) the order-disorder critical point. That is, an imposed shear acts as a field in a system that can order. Therefore, as  $\alpha \rightarrow 0^-$  and  $p_0 \rightarrow 0^+$ , the terms containing  $\lambda$  do not vanish; the relaxation rate is  $\sim q_\perp$  in this limit. From this, we expect the polar order to set in continuously. We can also use this to calculate the relevance of nonlinearities in this for this order-disorder transition. Because there is no anisotropy in the limit of  $\alpha \rightarrow 0$  (since rotation symmetry is broken spontaneously), we need to rescale space isotropically:  $x, y \rightarrow bx, by$ . The other rescalings are  $t \rightarrow b^z t$  and  $\mathbf{p} \rightarrow b^\chi \mathbf{p}$  where  $z$  is the dynamical exponent and  $\chi$  is the roughness exponent. Since the relaxation rate of polarisation fluctuations in the limit  $\alpha \rightarrow 0$  is  $\propto |q_\perp|$ ,  $z = 1$ . Holding the fluctuations of the order parameter fixed under renormalisation in the limit  $\alpha \rightarrow 0$  also requires holding the noise strength fixed. The noise strength under renormalisation scales as  $\Delta \rightarrow b^{z-2-2\chi} \Delta$  which implies  $\chi = -1/2$ . Using these *linear* exponents, it is immediately seen that the nonlinearity  $\mathbf{p} \cdot \nabla \mathbf{p}$  is irrelevant. In fact, the *only* nonlinearity that may be relevant is the usual  $p^2 \mathbf{p}$  cubic nonlinearity. Even this nonlinearity is only marginal (i.e.,  $d = 2$  is the critical dimension of this problem), implying that the critical exponents may not change from the linear ones predicted here. The fact that no nonlinearity – other than the cubic one arising from the potential – is even marginal is another consequence of long-range fluid-mediated interactions. Further, since all terms in the equation of motion that are *not invariant* under  $\mathbf{p} \rightarrow -\mathbf{p}$  turn out to be irrelevant, the universality class of this isotropic to polar transition and that of the isotropic-nematic transition in the NNC model discussed in Supp. E must be the same.

## Appendix I: Higher order corrections to the angular dynamics equations

In this supplementary section, I calculate the higher-order correction to the angular dynamics alluded to in the main text and in Supp. E and H for the NNC and PNC models respectively, and present an explicit expression for  $K_r$ . I first calculate this for the NNC model (nematic) and next, for the PNC model (polar).

### 1. Nematic

The correction to the Frank elastic coefficient in a nematic i.e., the  $\mathcal{O}(q_\perp^2)$  correction to  $-\Gamma_\theta K q_\perp^2$  passive term in (E2) arising from the fluid coupling is purely active. It arises from expanding the mobility (B17) to  $\mathcal{O}(q_\perp^0)$ . Using (B17) and the active stress (D4), the  $\mathcal{O}(q_\perp^2)$  term in (E2) is  $-\Gamma_\theta K_r(\phi) q_\perp^2 \theta$  where

$$K_r = K + \frac{\zeta}{32\eta\Gamma_\theta} [8\ell_s \cos 2\phi - \lambda\{\ell_b + 5\ell_s - (\ell_b - 3\ell_s) \cos 4\phi\}]. \quad (\text{I1})$$

That is, a non-zero Saffmann-Delbück length yields an active correction to the effective Frank elasticity. This activity-renormalised elasticity controls the wavelength of the fastest growing mode when the nematic state is linearly unstable.

The lowest-order passive correction to the angular dynamics due to the coupling with the fluid arises only at  $\mathcal{O}(q_\perp^3)$ . The linearised passive surface force density due to director distortions is

$$\mathbf{f}_p^s = -\frac{1+\lambda}{2} \partial_y \nabla_\perp^2 \theta \hat{x} + \frac{1-\lambda}{2} \partial_x \nabla_\perp^2 \theta \hat{y}. \quad (\text{I2})$$

This yields  $\mathcal{O}(q_\perp^3)$  term in the angular dynamics equation

$$-\frac{[q_x^4(\lambda-1)^2 + q_y^4(\lambda+1)^2 + 2q_x^2 q_y^2]}{8\eta|q_\perp|^3} K q_\perp^2 \theta, \quad (\text{I3})$$

which is obviously always stabilising. Using (C9), I now show that the static structure factor of angular fluctuations reduces to its equilibrium value, despite the coupling to the fluid, in the absence of activity. In a passive system, the angular fluctuations equation is

$$\partial_t \theta = - \left[ \frac{[q_x^4(\lambda-1)^2 + q_y^4(\lambda+1)^2 + 2q_x^2 q_y^2]}{8\eta|q_\perp|^3} + \Gamma_\theta \right] K q_\perp^2 \theta + \bar{\xi} + \xi \quad (\text{I4})$$

Taking  $\Delta = \Gamma_\theta T$  and  $\Delta^v = \eta T$ , where  $T$  is the temperature, as is required for passive systems,

$$\langle \bar{\xi}(\mathbf{q}_\perp, t) \bar{\xi}(\mathbf{q}'_\perp, t) \rangle + \langle \xi(\mathbf{q}_\perp, t) \xi(\mathbf{q}'_\perp, t) \rangle = 2T \delta(\mathbf{q}_\perp + \mathbf{q}'_\perp) \delta(t - t') \left[ \frac{[q_x^4(\lambda-1)^2 + q_y^4(\lambda+1)^2 + 2q_x^2 q_y^2]}{8\eta|q_\perp|^3} + \Gamma_\theta \right]. \quad (\text{I5})$$

This clearly follows the fluctuation-dissipation relation since the noise correlator is  $2T$  times the dissipative coefficient in front of  $\delta F / \delta \theta = K q_\perp^2 \theta$  in (I4) and the angular static structure factor is

$$\langle |\theta(\mathbf{q}_\perp, t)|^2 \rangle = \frac{T}{K q_\perp^2}. \quad (\text{I6})$$

This demonstrates that the long-range order of nematics is a consequence of activity – a passive nematic at an interface between two fluids only has quasi-long-range order and its static correlator can be calculated from the equipartition theorem (as for all equilibrium systems).

### 2. Polar

The angular dynamics in a polar state have both relaxational and propagating parts both at  $\mathcal{O}(q_\perp)$  (H1) and at  $\mathcal{O}(q_\perp^2)$ . The dissipative part at  $\mathcal{O}(q_\perp^2)$  is  $-\Gamma_p K_r^p(\phi) q_\perp^2 \theta$  where  $K_r^p(\phi)$  has the same expression as  $K_r$  in (I1), with  $\Gamma_\theta$  replaced by  $\Gamma_p$ . The  $\mathcal{O}(q_\perp^2)$  correction to the propagative part of the angular dynamics arises from the polar active stress with the coefficient  $\zeta_p$  (D6) which leads to a surface force density  $\zeta_p [\partial_x \partial_y \theta \hat{x} + (\partial_x^2 + 2\partial_y^2) \theta \hat{y}]$ . This, along with the  $\mathcal{O}(q_\perp^{-1})$  part of (B17) leads to a correction to  $v_p$  in (E2):  $v_p \rightarrow v_p + \zeta_p |q_\perp| (1 - \lambda) / 4\eta$ .

## Appendix J: Details of generic instability in the NC model

In this supplementary section, I detail the calculations that demonstrate that a homogeneous nematic phase formed by active nematogens constrained to float on the surface of a fluid or at a two-fluid interface, is generically unstable. This situation is described by the NC model in a state with perfect nematic order,  $S_0 = 1$ , and a mean concentration  $c_0$ . Expanding the osmotic pressure in (D9)  $\Pi_c(c) \approx A_r(c_0)\delta c$  to linear order in fluctuations about  $c_0$  and the active force  $\nabla_\perp \cdot (\zeta(c)\mathbf{Q}) \approx \zeta(c_0)(\partial_y\theta\hat{x} + \partial_x\theta\hat{y}) + \zeta_1(c_0)(\partial_x\delta c\hat{x} - \partial_y\delta c\hat{y})$  to linear order in  $\theta$  and  $\delta c$ , where  $\zeta_1 = (1/2)\partial_c\zeta(c)|_{c=c_0}$ , and solving for the velocity field I obtain the coupled equations of motion for the angle field from (D7) and the in-plane concentration from (D8) to leading order in wavenumbers:

$$\partial_t\theta = -\frac{\zeta}{4\eta}\frac{q_x^4(\lambda-1) + q_y^4(\lambda+1)}{|q_\perp|^3}\theta - \frac{q_xq_y[q_x^2\{A_r\lambda - (\lambda-2)\zeta_1\} + q_y^2\{A_r\lambda + (\lambda+2)\zeta_1\}]}{4\eta|q_\perp|^3}\delta c + \xi, \quad (\text{J1})$$

and

$$\partial_t\delta c = -\frac{\zeta c_0 q_x q_y}{2\eta|q_\perp|}\theta - \frac{c_0 q_x^2(A_r + \zeta_1) + c_0 q_y^2(A_r - \zeta_1)}{4\eta|q_\perp|}\delta c. \quad (\text{J2})$$

Here all coefficients such as  $\zeta$ ,  $\lambda$  are evaluated at  $c_0$  and both the conserving noise that vanishes at small wavenumbers as  $q_\perp^2$  and the noise from the coupling to the velocity field which scales as  $|q_\perp|$  (see Supp. C) have been suppressed in (J2) since they turn out to be irrelevant. The lowest order in wavenumber terms displayed in (J2) all arise from  $\nabla_\perp \cdot \mathbf{v}$  which is non-zero since there is no constraint of *in-plane* incompressibility. That is, at this order, the dynamics of the concentration field is slaved to the compression or dilation of the flow field. The diffusive terms appear only at the next order in wavenumbers  $\mathcal{O}(q_\perp^2)$  and, therefore, have been ignored in writing (J2). The eigenfrequencies of the coupled concentration and angular dynamics, from (J1) and (J2) are

$$\omega_\pm = -\frac{i|q_\perp|}{8\eta} \left[ (A_r + \zeta_1 \cos 2\phi)c_0 - \zeta \cos 2\phi(1 - \lambda \cos 2\phi) + \frac{\zeta\lambda}{2} \sin^2 2\phi \right. \\ \left. \pm \sqrt{\left\{ (A_r + \zeta_1 \cos 2\phi)c_0 - \zeta \cos 2\phi(1 - \lambda \cos 2\phi) + \frac{\zeta\lambda}{2} \sin^2 2\phi \right\}^2 + 4c_0\zeta\{\zeta_1 + A_r \cos 2\phi\}(1 - \lambda \cos 2\phi)} \right]. \quad (\text{J3})$$

For  $A_r \neq 0$ , at least one of the eigenfrequencies has a positive imaginary part for some  $\phi$  (except in a special case discussed in Supp. K), implying that the homogeneous nematic phase is *generically* destabilised in the NC model. In particular, for large  $A_r c_0 \gg \zeta, \zeta_1$ , which can be accessed by enhancing the concentration of active units, the film becomes essentially incompressible [53] since the dynamics is extremely sensitive to departures of  $c$  from  $c_0$ . In this case,  $\omega_+ = -(ic_0/4\eta)A_r|q_\perp|$  signals an infinitely fast relaxation of the concentration fluctuations as  $A_r \rightarrow \infty$  and  $\omega_- = (i\zeta/4\eta)|q_\perp| \cos 2\phi(1 - \lambda \cos 2\phi)$  reduces to the eigenfrequency obtained for the dynamics of the angle field in an incompressible two-dimensional interfacial layer [26–28, 35] which has the same angular character as the Simha-Ramaswamy instability [6]. The works of [26–28, 35] model a popular active matter system consisting of a thin layer of motors and microtubules at an oil-water interface, which was shown to be essentially incompressible in two dimensions [55]. This calculation demonstrates that the effective incompressibility is due to the high concentration of motors and microtubules (or motors, microtubules and surfactants) in that experiment.

At low  $A_r$ , the character of the generic instability diverges from the Simha-Ramaswamy instability. First, for  $A_r = 0$ ,  $\omega_-$  vanishes to  $\mathcal{O}(q_\perp)$  (i.e.,  $\omega_- \sim q_\perp^2$  and is controlled by the diffusivity and is, therefore, stabilising) while  $\omega_+$  has the same value as the eigenfrequency in (E2) to  $\mathcal{O}(q_\perp)$ , and is stable along all wavevector directions for  $\zeta\lambda > 0$  and  $|\lambda| > 0$  since the equation for angular fluctuations is decoupled from that of the concentration fluctuations at  $\mathcal{O}(q_\perp)$ . This implies that nematic order at the interface is stable in the NC model *only* in the limit of *infinite* compressibility in the NC model. At small but non-zero  $A_r \rightarrow 0$ ,  $\omega_-$  is generically *unstable* and increases linearly with  $A_r$ :

$$\lim_{A_r \rightarrow 0} \omega_- = \frac{iA_r c_0 |q_\perp|}{8\eta} \left[ -1 - \frac{\lambda - 4 \cos 2\phi + 3\lambda \cos 4\phi}{-4 \cos 2\phi + \lambda(3 + \cos 4\phi)} \right], \quad (\text{J4})$$

where, for simplicity, I have additionally taken  $\zeta_1 = 0$ , which doesn't qualitatively affect the discussion. Importantly, this eigenfrequency becomes *independent* of  $\zeta$  and, therefore, of its sign, at small  $A_r$  (i.e., when  $\zeta\lambda \gg A_r c_0$ . Of course,  $\omega_-$  vanishes when  $\zeta = 0$ ). The R.H.S. of (J4) vanishes generically for  $\phi = \pi/4$  implying that it is unstable even at small  $A_r$  either for  $\phi \gtrsim \pi/4$  or for  $\phi \lesssim \pi/4$  depending only on the value of  $\lambda$ . The crossover of  $\omega_-$  from being

independent of  $\zeta$  when  $\zeta\lambda \gg A_r c_0$  to linearly depending on  $\zeta$  when  $\zeta\lambda \ll A_r c_0$  is best examined by expanding (J3) (still in the simplifying  $\zeta_1 = 0$  limit) near  $\phi = \pi/4$ :

$$\omega_-(\phi \approx \pi/4) \approx -\frac{i|q_\perp|}{\eta} \frac{A_r c_0 \zeta}{2A_r c_0 + \zeta\lambda} \left(\phi - \frac{\pi}{4}\right). \quad (\text{J5})$$

This clearly demonstrates that at small  $A_r$ ,  $\omega_-$  is independent of  $\zeta$  but depends on  $A_r$  and, as the concentration is increased at a fixed activity, it ceases to depend on  $A_r$  beyond a critical value  $\propto \zeta\lambda$ . This instability of an interfacial nematic phase in the NC model bears a strong conceptual analogy with the instability of a *compressible* nematic state in a *momentum-conserved* fluid described in Supp. L (this is an extension of the Simha-Ramaswamy instability). In particular, the angular character of the two instabilities is essentially analogous. This demonstrates that the lack of incompressibility of the interfacial layer is not enough to ensure the stability of an interfacial ordered nematic state. Instead, the exchange of active units between the interface and the bulk is essential for order. Note that  $\omega_+$  is not generically destabilising near  $\phi = \pi/4$ :

$$\omega_+(\phi \approx \pi/4) \approx -\frac{i|q_\perp|}{2} \left[ \frac{2A_r c_0 + \zeta\lambda}{4\eta} + \frac{\zeta^2 \lambda}{2A_r c_0 \eta + \zeta\eta\lambda} \left(\phi - \frac{\pi}{4}\right) \right] \quad (\text{J6})$$

and does not vanish in the  $A_r = 0$  limit, instead going to a constant value which is stabilising for all  $\phi$  when  $\zeta\lambda > 0$ .

Throughout this calculation, I have assumed that  $A_r \geq 0$ , i.e., the osmotic pressure is stabilising. Therefore, the destabilisation described in this section is associated with a state with nematic order. Indeed, a disordered state of elongated, active particles is *not* unstable to incipient order, unlike bulk extensible active systems. The velocity couplings in this system enter the order parameter equation at  $\mathcal{O}(q_\perp)$  and, therefore, cannot compete against the wavenumber-independent relaxation of the order parameter magnitude in the disordered state. As long as  $A_r \geq 0$ , a collection of *isotropic* active swimmers is also immune to a small wavenumber instability towards phase separation. In this case, the only hydrodynamic variable is the concentration of the active particle  $c$  and, to the lowest order in wavenumbers, its eigenfrequency is  $\omega_c = -iA_r|q_\perp|/4\eta + \mathcal{O}(q_\perp^2)$ . Conversely, this implies an osmotic pressure-induced instability towards phase separation of isotropic swimmers at fluid interfaces when the osmotic pressure is destabilising i.e.,  $A_r < 0$ . This is distinct from phase-separation mechanisms identified in active model H [4, 5]; there, osmotic pressure cannot induce phase separation due to incompressibility. The consequences of this osmotic pressure-induced instability, which is unique to interfacial swimmers, will be examined elsewhere.

### Appendix K: Stable interfacial nematic composed of particles living at the interface

In this supplementary section, I show that there is a special point in the parameter space at which a stable nematic phase exists in the NC model. This special point is accessed when  $A_r > |\zeta_1|$ ,  $\lambda = -A_r/\zeta_1$  and  $\zeta\zeta_1 < 0$ . In this case, the eigenfrequencies become

$$\omega_\pm = -\frac{i|q_\perp|}{8\eta} \left[ (c_0\zeta_1 - \zeta) \cos 2\phi + c_0 A_r - \frac{A_r \zeta}{2\zeta_1} (1 + \cos^2 2\phi) \right. \\ \left. \pm \sqrt{\left\{ (\zeta - c_0\zeta_1) \cos 2\phi - c_0 A_r + \frac{A_r \zeta}{2\zeta_1} (1 + \cos^2 2\phi) \right\}^2 + 4 \frac{c_0 \zeta}{\zeta_1} \{\zeta_1 + A_r \cos 2\phi\}^2} \right]. \quad (\text{K1})$$

It is clear that when  $A_r > |\zeta_1|$  and  $\zeta\zeta_1 < 0$ , the term inside the square bracket and outside the square root is positive while the magnitude of the term inside the square root is smaller than the term outside the square root (since  $\zeta\zeta_1 < 0$ ). Therefore, both  $\omega_\pm$  have negative imaginary parts for all  $\phi$  in this case, implying stability. However,  $\omega_-$  is 0 for some specific  $\phi$ . In these directions, the eigenfrequency is  $\mathcal{O}(q_\perp^2)$ . This feature makes the properties of this nematic phase distinct from the one in Sec. III of the main text or Supp. E as can be seen from the scaling of the static structure factors of angular and concentration fluctuations. Upon defining  $\kappa_+ = i\omega_+$  and  $\kappa_- = i\omega_- + \bar{K}(\phi)q_\perp^2$ , where  $\bar{K}$  is the  $\mathcal{O}(q_\perp^2)$  part of the eigenfrequency, the dynamic structure factor of angular fluctuations reads

$$\langle |\theta(\mathbf{q}_\perp, \omega)|^2 \rangle = \frac{2[\omega^2 + c_0^2 q_\perp^2 (A_r + \zeta_1 \cos 2\phi)^2] \Delta}{16\eta^2 (\omega^2 + \kappa_+^2) (\omega^2 + \kappa_-^2)} \quad (\text{K2})$$

which yields the static structure factor

$$\langle |\theta(\mathbf{q}_\perp, t)|^2 \rangle = \frac{\Delta}{16\eta^2 (\kappa_+ + \kappa_-)} + \frac{\Delta c_0^2 q_\perp^2 (A_r + \zeta_1 \cos 2\phi)^2}{16\eta^2 \kappa_1 \kappa_2 (\kappa_+ + \kappa_-)}. \quad (\text{K3})$$

The first term in (K3) scales as  $\sim 1/|q_\perp|$  along all directions since  $\kappa_+ + \kappa_-$  has a non-vanishing  $\mathcal{O}(q_\perp)$  term along all wavevector directions. The second term, however, scales as  $\sim 1/q_\perp^2$  along directions in which the  $\mathcal{O}(q_\perp)$  part of  $\kappa_-$  vanishes (the numerator never vanishes since  $A_r > |\zeta_1|$ ). The real-space angular fluctuations are calculated as  $\langle |\theta(\mathbf{r}_\perp, t)|^2 \rangle = \int d^2 q_\perp \langle |\theta(\mathbf{q}_\perp, t)|^2 \rangle / 4\pi^2$ . This integral is clearly dominated by the points where  $\kappa_-$  is  $\mathcal{O}(q_\perp^2)$ . This happens at a  $\phi = \phi_0$  that depends on the ratio of  $A_r/\zeta_1$ . Expanding  $\kappa_- = A_1(\delta\phi)^2|q_\perp| + \bar{K}(\phi_0)q_\perp^2$  around these points where  $\delta\phi = \phi - \phi_0$  and  $A_1$  is a constant whose value depends on  $\zeta$ ,  $A_r$  and  $\zeta_1$ , I obtain

$$\langle |\theta(\mathbf{r}_\perp, t)|^2 \rangle \approx S \int |q_\perp| d|q_\perp| \int_{-\infty}^{\infty} d\delta\phi \frac{1}{(\delta\phi)^2|q_\perp| + B^2|q_\perp|^2} \quad (\text{K4})$$

where  $S$  and  $B$  are constants. I have extended the range of the angular integral to  $\pm\infty$  since it is dominated by  $\delta\phi \ll 1$ . The angular integral evaluates to

$$\int_{-\infty}^{\infty} d\delta\phi \frac{1}{(\delta\phi)^2|q_\perp| + B^2|q_\perp|^2} = \frac{\pi}{B|q_\perp|^{3/2}} \quad (\text{K5})$$

and, therefore,  $\langle |\theta(\mathbf{r}_\perp, t)|^2 \rangle \propto \int q_\perp^{-1/2} d|q_\perp|$  which clearly converges in the long wavelength limit, implying long-range order. However, unlike the nematic state in Sec. III of the main text or Supp. E, this implies a roughness exponent  $\chi = -1/4$  and not  $\chi = -1/2$ . Since the static structure factor is not isotropically  $1/|q_\perp|$  in all directions, the anisotropy and dynamical exponents are also not 1.

The static structure factor of concentration fluctuations can be calculated similarly:

$$\langle |\delta c(\mathbf{q}_\perp, t)|^2 \rangle = \frac{\zeta^2 c_0^2 \sin^2 2\phi \Delta |q_\perp|^2}{16\eta^2 (\kappa_+^2 \kappa_- + \kappa_-^2 \kappa_+)}, \quad (\text{K6})$$

implying real space concentration fluctuations  $\langle |\delta c(\mathbf{r}_\perp, t)|^2 \rangle \propto \int q_\perp^{-1/2} d|q_\perp|$ . This implies that the R.M.S. number fluctuations,  $\sqrt{\langle \delta N \rangle^2}$ , in a region containing on average  $\langle N \rangle$  particles, scales as  $\langle N \rangle^{7/8}$ . Since the angular fluctuations are *softer* than  $1/|q_\perp|$ , the concentration fluctuations are larger than  $\langle N \rangle^{3/4}$  found for a polar flock composed of interface-associated swimmers in the PC model (see sec. IV of the main text and Supp. M). However, the nematic phase discussed in this section requires a perfect tuning of parameter values and is unlikely to be realised in any experimental system.

## Appendix L: Bulk, momentum-conserved, compressible active fluids

A natural question that arises from the discussion of aligned interfacial states is precisely what allows such states to escape the Simha-Ramaswamy instability. Is it the mere fact that an interface is not incompressible (in two dimensions)? The generic instability of the aligned state in the NC model at *any* finite compressibility (see Sec. J) suggests that is not the case. In this section, I consider *compressible* momentum-conserved active fluids and show that nematic states are generically unstable for any finite compressibility. That is, bulk nematic order is generically destroyed in fluids in which mass and momentum are conserved. In polar fluids, this Simha-Ramaswamy instability is cut-off by self-advection as was shown (for an incompressible fluid) in [56].

For simplicity and notational continuity, I consider a two-dimensional, momentum-conserved active fluid, though the result (i.e., that a nematic state is generically unstable) can be easily shown to hold in all dimensions. The linearised equations of motion for fluctuations of a bulk, compressible active nematic read, to the lowest order in gradients,

$$\partial_t \delta \rho = -\rho_0 \nabla_\perp \cdot \mathbf{v}, \quad (\text{L1})$$

$$\partial_t \theta = \frac{1-\lambda}{2} \partial_x v_y - \frac{1+\lambda}{2} \partial_y v_x \quad (\text{L2})$$

and

$$\rho_0 \partial_t \mathbf{v} = \eta \nabla_\perp^2 \mathbf{v} - A_r \nabla_\perp \delta \rho - \zeta (\partial_x \theta \hat{y} + \partial_y \theta \hat{x}), \quad (\text{L3})$$

where  $\rho$  is the density with  $\rho_0$  being its mean value and  $A_r$  is the inverse compressibility. One of the eigenfrequencies of this system of equations is *always* destabilising for  $A_r \neq 0$ . This is simplest to demonstrate in the Stokes limit in



which viscous forces are balanced by other forces in the limit of small Reynolds number. In this case, the equations of motion for  $\delta c$  and  $\theta$  read, after eliminating the velocity field

$$-i\omega\delta\rho = -\frac{\rho_0 A_r}{\eta}\delta\rho - \frac{\rho_0\zeta\sin 2\phi}{\eta}\theta \quad (\text{L4})$$

and

$$-i\omega\theta = -\frac{\zeta(\lambda - \cos 2\phi)}{2\eta}\theta - \frac{A_r\lambda\sin 2\phi}{2\eta}\delta\rho. \quad (\text{L5})$$

It is clear that when  $A_r = 0$ , this pair of equations has only one non-zero eigenfrequency (at this order in wavenumbers)  $\omega_+ = -i\zeta(\lambda - \cos 2\phi)/2\eta$  which is stabilising when  $\zeta\lambda > 0$  and  $|\lambda| > 1$ . However, for any  $A_r > 0$ ,  $\omega_-$  is non-zero and is *destabilising*. The eigenvalues for arbitrary  $A_r$  are

$$\omega_{\pm} = -\frac{1}{4\eta} \left[ 2\rho_0 A_r + \zeta(\lambda - \cos 2\phi) \pm \sqrt{\zeta^2(\lambda - \cos 2\phi)^2 + 4\rho_0 A_r \{\rho_0 A_r + \zeta(\cos 2\phi - \lambda \cos 4\phi)\}} \right] \quad (\text{L6})$$

Expanding (L6) for small  $A_r$ , I get

$$\lim_{A_r \rightarrow 0} \omega_- = \frac{A_r \rho_0 \cos 2\phi (1 - \lambda \cos 2\phi)}{\eta(\lambda - \cos 2\phi)}. \quad (\text{L7})$$

Just like Eq. (J4), the eigenfrequency (L7) also vanishes for  $\phi = \pi/4$  and changes sign as it passes through it, signifying a generic instability. Furthermore, again, like Eq. (J4), it also becomes independent of  $\zeta$  at small  $A_r$ . The fact that  $\omega_-$  always changes sign around  $\phi = \pi/4$  can be seen by expanding (L6) about  $\pi/4$ :

$$\omega_-(\phi \approx \pi/4) = -\frac{i\rho_0}{\eta} \frac{2A_r\zeta}{2A_r\rho_0 + \zeta\lambda} \left( \phi - \frac{\pi}{4} \right). \quad (\text{L8})$$

The form of this is similar to (J5) in Sec. J (except that there, the eigenfrequency scales as  $\sim |q_{\perp}|$ ).

In polar systems, in addition, (L1) contains extra linear terms  $\propto \partial_x \delta\rho$  and  $\partial_y \theta$  and (L2) contains terms  $\propto \partial_y \delta\rho$  and  $\partial_x \theta$ . However, in the strict Stokesian limit discussed above, these do not affect the  $\mathcal{O}(q_{\perp}^0)$  part of the eigenvalue and cannot modify the small wavenumber instability. That is, in the Stokesian limit, both active nematic and polar order are generically unstable even in compressible systems.

Note that the instability of the *nematic* phase does not require Stokesian dynamics. In other words, active nematic order is not saved by inertia [6]. To show this, I now calculate the mode structure implied by (L1), (L2) and (L3) by dropping the viscous term. This yields two pairs of propagating modes

$$\omega = \pm \frac{q_{\perp}}{2\sqrt{\rho_0}} \sqrt{2\rho_0 A_r + \zeta(\lambda - \cos 2\phi) \pm \sqrt{\zeta^2(\lambda - \cos 2\phi)^2 + 4\rho_0 A_r \{\rho_0 A_r + \zeta(\cos 2\phi - \lambda \cos 4\phi)\}}}. \quad (\text{L9})$$

Notice that the term inside the large square root is *exactly* the same as the term in the square brackets in (L6). When  $A_r = 0$ , the speed for a pair of modes vanishes and the other pair has a dispersion relation

$$\omega_{\pm}^{(1)} = \pm \frac{q_{\perp}}{\sqrt{2\rho_0}} \sqrt{\zeta(\lambda - \cos 2\phi)}. \quad (\text{L10})$$

The wave speed is real and the ordered state is not destabilised when  $\zeta\lambda > 0$  and  $|\lambda| > 1$ . For small  $A_r$ , the second pair of sound modes has a non-zero speed:

$$\lim_{A_r \rightarrow 0} \omega_{\pm}^{(2)} = \pm q_{\perp} \sqrt{A_r} \sqrt{\frac{\cos 2\phi(\lambda \cos 2\phi - 1)}{\lambda - \cos 2\phi}}. \quad (\text{L11})$$

Again, in the small  $A_r$  limit, this wave speed is independent of  $\zeta$ . As  $\phi$  passes through  $\pi/4$ , the term in the second square root changes sign; i.e., the wave speed becomes imaginary, signifying an instability. This happens at arbitrary  $A_r$  as can be seen by expanding (L9) around  $\phi = \pi/4$ . Doing that, I find

$$\omega_{\pm}^{(2)}(\phi \approx \pi/4) = \pm q_{\perp} \sqrt{\frac{2A_r\zeta}{2\rho_0 A_r + \zeta\lambda}} \left( \phi - \frac{\pi}{4} \right), \quad (\text{L12})$$

clearly showing that the speed of this pair of modes is imaginary either for  $\phi > \pi/4$  or for  $\phi < \pi/4$  signifying a generic instability.

In polar systems, in contrast, self-advection (i.e., a term  $\propto \partial_x \theta$  in (L2)) cuts off the instability in analogy with the stabilisation described in incompressible systems by [56].

The phenomenology of the instability in the NC model is analogous to the instability described here for active nematic compressible fluid. This instability is averted in the NNC model because the *number* of active units at the interface is not conserved there. The analogous instability is averted at high motilities in the PC model via a mechanism that is somewhat similar to that by which highly motile polar fluids escape the instability described here (although in the PC model, the instability is averted even in the strict Stokesian limit).

### Appendix M: Details of motility-driven ordering in the PC model

In this supplementary section, I present the detailed calculations demonstrating that a polar species living at the surface can outrun the instability that plagues its immotile cousins (the NC model) and form stable, motile ordered states at fluid-fluid or fluid-air interfaces of momentum-conserved systems, as discussed in Sec. IV of the main text. Solving for the velocity field using (B18) and (D12) and expanding the equations of motion of the polarisation field (D10) and the concentration field (D11) of the PC model of Supp. D in angular fluctuations  $\theta$  about a perfectly ordered state with  $p_0 = 1$  and  $\delta c$  – the local deviation of the concentration field about its mean value  $c_0$  – to leading order in wavenumbers yields

$$\partial_t \theta = -\frac{\zeta}{4\eta} \frac{q_x^4(\lambda - 1) + q_y^4(\lambda + 1)}{|q_\perp|^3} \theta - \frac{q_x q_y [q_x^2 \{A_r \lambda - (\lambda - 2)\zeta_1\} + q_y^2 \{A_r \lambda + (\lambda + 2)\zeta_1\}]}{4\eta |q_\perp|^3} \delta c - i\Gamma_p \gamma q_y \delta c - i v_p q_x \theta + \xi, \quad (\text{M1})$$

and

$$\partial_t \delta c = -\frac{\zeta c_0 q_x q_y}{2\eta |q_\perp|} \theta - \frac{c_0 q_x^2 (A_r + \zeta_1) + c_0 q_y^2 (A_r - \zeta_1)}{4\eta |q_\perp|} \delta c - i \bar{v}_c q_x \delta c - i v_c q_y \theta. \quad (\text{M2})$$

Here, as in Supp. J,  $\zeta_1 = (1/2)\partial_c \zeta(c)|_{c=c_0}$ .  $\bar{v}_c$  is defined as  $\bar{v}_c = \partial_c [c v_c(c)]|_{c=c_0}$ . The noise in the concentration equation is ignored since it turns out to be irrelevant as I will explicitly demonstrate post-facto (see also Supp. C). I now examine the mode structure implied by (M1) and (M2) in some limits. First, when  $A_r c_0 \gg \zeta, \zeta_1, \bar{v}_c \eta, v_p \eta$ , the active system is effectively incompressible and as in the NC model (see Supp. J), the imaginary part of one of the two eigenfrequencies diverge with  $A_r c_0$ , signifying an infinitely fast relaxation of the concentration fluctuations while the imaginary part of the other eigenvalue, to  $\mathcal{O}(q_\perp)$ , has the angular character of the Simha-Ramaswamy instability implying a generic destruction of the ordered state in the PC model:

$$\omega_+ = \left[ \left( \bar{v}_c + \frac{v_c \lambda}{c_0} \sin^2 \phi \right) \cos \phi - \frac{i c_0}{4\eta} A_r \right] |q_\perp|, \quad (\text{M3})$$

$$\omega_- = \left[ \left( v_p - \frac{v_c \lambda \sin^2 \phi}{c_0} \right) \cos \phi + \frac{i \zeta}{4\eta} (\cos 2\phi - \lambda \cos^2 2\phi) \right] |q_\perp|. \quad (\text{M4})$$

However, unlike in the NC model, the ordered state is not unstable in the entire parameter range of the PC model. Specifically, for large  $v_p$  or large  $\bar{v}_c$  (i.e., for  $v_p, \bar{v}_c \gg A_r c_0 / \eta$ ), disturbances can outrun the exponential growth, stabilising the ordered phase. In both limits, the eigenfrequencies for all  $\phi \neq (2n + 1)\pi/2$ , where  $n$  is an integer, the eigenfrequencies to leading order in  $v_p$  and  $\bar{v}_c$  are

$$\omega_+ = \left[ \bar{v}_c \cos \phi - i \frac{c_0}{4\eta} (A_r + \zeta_1 \cos 2\phi) \right] |q_\perp| \quad (\text{M5})$$

and

$$\omega_- = \left[ v_p \cos \phi + \frac{i \zeta}{4\eta} \left( \cos 2\phi - \lambda \cos^2 2\phi - \frac{\lambda}{2} \sin^2 2\phi \right) \right] |q_\perp|. \quad (\text{M6})$$

This implies that for  $\zeta_1 \ll A_r$  both of these eigenfrequencies are stabilising when  $|\lambda| > 1$  and  $\zeta \lambda > 0$ . Of course the closer  $\phi$  is to  $\pi/2$ , the large  $v_p$  or  $\bar{v}_c$  must be for the expansion to hold. For the ordered state to be stable, the

fluctuations along  $\phi = (2n + 1)\pi/2$

$$\omega_{\pm}(\phi = \pi/2) = -\frac{i|q_{\perp}|}{8\eta} \left[ (A_r - \zeta_1)c_0 + \zeta(1 + \lambda) \pm \sqrt{\{\zeta(1 + \lambda) - (A_r - \zeta_1)c_0\}^2 - 64v_c\gamma\eta^2} \right]. \quad (\text{M7})$$

must also be stabilising. Indeed, these eigenfrequencies are *not* generically destabilising i.e., the imaginary part of either of these is not generically positive; in particular, they are stabilising when  $\gamma v_c > 0$ ,  $\zeta\lambda > 0$  and  $|\lambda| > 1$ . This is the advertised outrunning of the active instability by motility which implies a stable interfacial polar state in the PC model even when the motile particles are localised at the interface. The mechanism for the survival of a polar phase in the PC model has conceptual similarities to the suppression of the bulk instability in extensile polar fluids due to *inertia* [56].

The stability boundary of the polar phase is best examined in a simplifying limit  $\bar{v}_c = 0$ ,  $v_c = 0$ ,  $\gamma = 0$  and  $\zeta_1 = 0$ , in terms of the non-dimensional parameters  $\mathcal{R}_1 = A_r c_0 / 4v_p \eta$  and  $\mathcal{R}_2 = \zeta / 4v_p \eta$ . The eigenfrequencies, in terms of  $\mathcal{R}_1$  and  $\mathcal{R}_2$ , for all values of  $v_p$ , are

$$\omega_{\pm} = \frac{i|q_{\perp}|v_p}{2} \left[ \mathcal{S}(\phi) \pm \sqrt{\mathcal{S}(\phi)^2 - 4\mathcal{R}_1\{i \cos \phi - \mathcal{R}_2 \cos 2\phi(1 - \lambda \cos 2\phi)\}} \right]. \quad (\text{M8})$$

where  $\mathcal{S}(\phi) = -\mathcal{R}_1 + \mathcal{R}_2[\cos 2\phi - \lambda(1 + \cos^2 \phi)/2] - i \cos \phi$ . In the limit of large  $v_p$ , i.e., when  $\mathcal{R}_1, \mathcal{R}_2 \ll 1$ , the term  $\propto \cos^2 \phi$  appearing from  $\mathcal{S}(\phi)^2$  dominates inside the square root when  $\cos \phi \neq 0$ , yielding (M5) and (M6) (with  $v_c = \bar{v}_c = \zeta_1 = 0$ ). The stability boundary of the polar phase depends on the non-dimensional parameters  $\mathcal{R}_1$ ,  $\mathcal{R}_2$  and  $\lambda$ . A representative plot of the stability region of the homogeneous polar phase in the  $\mathcal{R}_1, \mathcal{R}_2$  plane, for a specific choice of  $\lambda$  ( $\lambda = 2$ ) is displayed in the main text.

The stability of the polar phase for large advection speed is possible because the growth rate of the instability in the  $v_p \rightarrow 0$  limit is itself  $\sim q_{\perp}$  due to the momentum exchange between the layer and the bulk fluid. It cannot happen in a *bulk Stokesian* fluid where the growth rate is wavevector-independent [6, 56].

The static structure factor of angular fluctuations in the stable polar phase in the PC model scale as  $\sim 1/|q_{\perp}|$  in all directions of the wavevector space (as in the NNC and PNC models), implying long-range polar order in two dimensions. Restoring motility  $v_c \neq 0$ ,  $\bar{v}_c \neq 0$ , the dynamic structure factor of concentration fluctuations implied by (M1) and (M2) in the stable polar state is

$$\langle |\delta c(\mathbf{q}_{\perp}, \omega)|^2 \rangle = \frac{2(\zeta^2 c_0^2 \sin^2 2\phi + 16\eta^2 v_c^2 \sin^2 \phi) \Delta |q_{\perp}|^2}{16\eta^2 \{(\omega - c_+)^2 + \kappa_+^2\} \{(\omega - c_-)^2 + \kappa_-^2\}}, \quad (\text{M9})$$

where  $-\text{Im}[\omega_{\pm}] = \kappa_{\pm}$  and  $\text{Re}[\omega_{\pm}] = c_{\pm}$  with both  $c_{\pm}$  and  $\kappa_{\pm}$  being  $\mathcal{O}(|q_{\perp}|)$ . Here,  $\Delta$  is the strength of the non-conserved noise in (M1) which enters the concentration equation via the motility and is dominant in the small wavenumber regime. Integrating  $\int_{-\infty}^{\infty} (d\omega/2\pi) \langle |\delta c(\mathbf{q}_{\perp}, \omega)|^2 \rangle$  over all frequencies yield the static structure factor of the concentration fluctuations:

$$\langle |\delta c(\mathbf{q}_{\perp}, t)|^2 \rangle = \frac{(\zeta^2 c_0^2 \sin^2 2\phi + 16\eta^2 v_c^2 p_0^2 \sin^2 \phi) \Delta |q_{\perp}|^2 (\kappa_+ + \kappa_-)}{16\eta^2 \kappa_+ \kappa_- \{(c_+ - c_-)^2 + (\kappa_+ + \kappa_-)^2\}} \propto \frac{1}{|q_{\perp}|}. \quad (\text{M10})$$

The  $1/|q_{\perp}|$  divergence of the static structure factor of concentration fluctuations implies that the R.M.S. number fluctuations  $\sqrt{\langle \delta N^2 \rangle}$  in a region with  $\langle N \rangle$  particles on average scales as  $\langle N \rangle^{3/4}$ , instead of as  $\langle N \rangle^{1/2}$  as it would in all equilibrium systems not at a critical point, and thus violates the law of large numbers. This implies giant number fluctuations – which had earlier been discussed both for polar and nematic active systems *in contact with substrates* [14, 19, 23, 24, 57] – even in this fully-momentum-conserved system. However, in the PC model, the divergence of the concentration static structure factor is milder ( $\sim 1/|q_{\perp}|$  instead of  $\sim 1/q_{\perp}^2$ ) than in systems on substrates and, as a result, the number fluctuations are less violent (though still larger than in equilibrium and, therefore, giant) due to the coupling of the two-dimensional film with the bulk fluid medium.

I now demonstrate that (M1) and (M2) also yield the *exact* exponents of the polar phase. The dynamical exponent  $z$ , the anisotropy exponent  $\mu$  and the roughness exponent  $\chi$  remain unchanged from the NNC model (see Sec. III of the main text or Supp. E):  $z = \mu = 1$ ,  $\chi = -1/2$ . Defining  $\chi_c$  as the exponent characterising the concentration fluctuations via  $\delta c \rightarrow b^{\chi_c} \delta c$ , it is clear from (M10) that  $\chi_c = -1/2$  as well. This is expected since (M1) and (M2) imply that concentration and angular fluctuations scale the same way. As in the NNC and PNC models, (Sec. III of the main text or Supp. E), there is no relevant nonlinearity: the lowest order nonlinearities, arising either from the flow couplings or advection or motility in either equation must scale as  $q_{\perp}(\theta^2)_{q_{\perp}}$ ,  $q_{\perp}(\delta c^2)_{q_{\perp}}$  or  $q_{\perp}(\delta c \theta)_{q_{\perp}}$  all of which are irrelevant.

As in Sec. J, I have assumed that the osmotic pressure is stabilising i.e.,  $A_r > 0$ . As is clear from (M5),  $A_r < 0$  i.e., an osmotic pressure which would promote an instability towards a phase-separated state in the absence of polar order, always destroys the homogeneous polar phase.

Next, I show that the inclusion of the noise term  $\bar{\xi}_c$  in the concentration equation, which was argued to be irrelevant in Sec. C (just below Eq. (C10)) doesn't modify the small wavenumber static structure factors of concentration and angular fluctuations. From Eq. (C10) the standard deviation of this noise is  $\mathcal{O}(q_\perp)$ . Using (C10), I obtain an additional part of the static structure factor for concentration fluctuations dependent on  $\bar{\xi}_c$ :

$$[\langle |\delta c(\mathbf{q}_\perp, \omega)|^2 \rangle]_{\Delta^v} = \frac{[16\eta^2(\omega - |q_\perp|v_p \cos \phi)^2 + \zeta^2 \mathcal{G}(\phi)^2 q_\perp^2] 2c_0^2 |q_\perp| \Delta^v}{64\eta^4 \{(\omega - c_+)^2 + \kappa_+^2\} \{(\omega - c_-)^2 + \kappa_-^2\}}, \quad (\text{M11})$$

where  $\mathcal{G}(\phi) = \cos 2\phi(\lambda \cos 2\phi - 1) + \lambda \sin^2 2\phi/2$ . Integrating this over all  $\omega$  yields the contribution of  $\Delta^v$  to the static structure factor  $[\langle |\delta c(\mathbf{q}_\perp, t)|^2 \rangle]_{\Delta^v}$  which, as expected, is wavenumber-independent (but is a complicated function of  $\phi$ ). Similarly, evaluating the contribution of the noise  $\bar{\xi}_c$  to the static structure factor of angular fluctuations, I find that it too is independent of wavenumber (but, again, a complicated function of  $\phi$ ). Therefore, these contributions to the static structure factor do not diverge at small wavenumber and are subdominant to the pieces of the static structure factor that diverge at small wavenumbers as  $1/|q_\perp|$ . This post-facto justifies neglecting  $\bar{\xi}_c$ .

Finally, I examine the disordered-polar transition in this PC model. In *dry* systems composed of a conserved number of polar particles on a substrate without an intervening fluid medium, the transition to the polarised phase is not continuous. Instead, a periodic array of propagating polar bands form in the disordered phase [54] which finally forms the homogeneous polar phase. While a detailed examination of this process is involved, an indication that the order-disorder transition is gleaned from the fact that an incipient homogeneous polar state turns out to be unstable in the limit  $\alpha \rightarrow 0^-$  (i.e., what would normally be the second order critical point) [14]. I examine the equivalent question for the disordered-polar transition in the PC model.

To do this, I expand the polarisation and concentration fluctuations about a homogeneous state:  $\mathbf{p} = (p_0 + \delta p)(\cos \theta, \sin \theta)$  with  $p_0 = \sqrt{|\alpha|/\beta} \neq 1$  and  $c = c_0 + \delta c$ . Crucially, since I am interested in understanding the properties of the disordered-polar transition, I need to retain both  $\delta p$  and  $\theta$  fluctuations as both are slow near the critical point. I now expand (D10) and (D11) about this state to linear order in  $(\delta p, \theta, \delta c)$ . To first order in wavenumbers, this yields

$$\begin{aligned} \partial_t \delta p = & -2|\alpha|\Gamma_p \delta p - ip_0|q_\perp|v_p \cos \phi \delta p - \frac{\lambda p_0^2 |q_\perp| (\zeta + 2|\alpha|\lambda)(3 - \cos 4\phi)}{16\eta} \delta p + \frac{p_0^3 \lambda \zeta |q_\perp| \sin 4\phi}{16\eta} \theta \\ & + ap_0\Gamma_p \delta c - i\gamma\Gamma_p |q_\perp| \cos \phi \delta c - \frac{p_0 |q_\perp| \lambda [4A_r \cos 2\phi + p_0^2 (\zeta_1 - 2a\lambda)(3 - \cos 4\phi)]}{32\eta} \delta c, \end{aligned} \quad (\text{M12})$$

$$\begin{aligned} \partial_t \theta = & -\frac{p_0 |q_\perp| \sin 2\phi (\zeta + 2|\alpha|\lambda)(2 - \lambda \cos 2\phi)}{8\eta} \delta p - ip_0|q_\perp|v_p \cos \phi \theta - \frac{p_0^2 |q_\perp| \zeta [\lambda(3 + \cos 4\phi) - 4 \cos 2\phi]}{16\eta} \theta \\ & - i\gamma\Gamma_p |q_\perp| \sin \phi \delta c - \frac{|q_\perp| \sin 2\phi [2\{A_r \lambda + p_0^2 (\zeta_1 - 2a\lambda)\} + p_0^2 \lambda \cos 2\phi (\zeta_1 - 2a\lambda)]}{16\eta} \delta c \end{aligned} \quad (\text{M13})$$

$$\begin{aligned} \partial_t \delta c = & -iv_c |q_\perp| \cos \phi \delta p - \frac{c_0 p_0 |q_\perp| (\zeta + 2|\alpha|\lambda) \cos 2\phi}{4\eta} \delta p - iv_c p_0 |q_\perp| \sin \phi \theta - \frac{c_0 p_0^2 \zeta \cos \phi \sin \phi}{2\eta} \theta \\ & - i\bar{v}_c p_0 |q_\perp| \cos \phi \delta c - \frac{c_0 |q_\perp| \{2A_r + p_0^2 (\zeta_1 - 2a\lambda) \cos 2\phi\}}{8\eta} \delta c \end{aligned} \quad (\text{M14})$$

To examine the stability of an incipient homogeneously ordered phase, I need to examine the stability of this system of equations in the limit  $p_0 \rightarrow 0^+$  and  $\alpha \rightarrow 0^-$ . In dry flocks, the instability appears along the ordering direction. Therefore, it is enough to examine the stability of the incipient ordered state even in this model for  $\phi = 0$ . Along this direction, the  $\theta$  field decouples from  $\delta p$  and  $\delta c$  and has the eigenfrequency

$$\omega_\theta = p_0 q_x v_p - i \frac{p_0^2 q_x \zeta (\lambda - 1)}{4\eta}. \quad (\text{M15})$$

One of the other two eigenfrequencies is damped at zeroth order in wavenumber  $\omega_p = -i2|\alpha|\Gamma_p$ . The third eigenfrequency is  $\mathcal{O}(q_\perp)$  unlike in dry flocks where this scales as  $\mathcal{O}(q_\perp^2)$ . Importantly, this eigenfrequency is *generically* destabilising in the limit  $\alpha \rightarrow 0^-$  in dry flocks signalling the existence of a microphase-separated state consisting

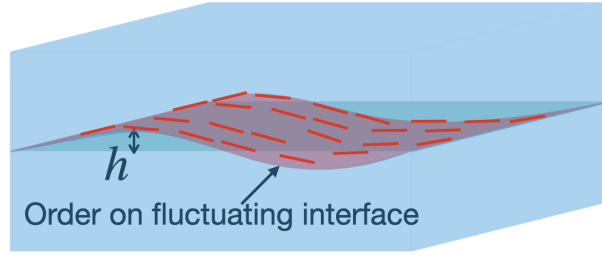

FIG. 1. Order on a fluctuating interface or immersed surface in a fluid. The small surface fluctuations are parametrised by the height field  $h$  which measures the local displacement of the surface from a flat, fiducial one.

of high-density, periodically organised travelling polar bands in a low-density, isotropic background. However, for interfacial flocks in the PC model, the imaginary part of the eigenfrequency

$$\lim_{|\alpha| \rightarrow 0^-} \text{Im}[\omega_c] = -\frac{c_0}{\eta} \left[ \frac{A_r}{4} + \frac{a\zeta}{8\beta} \right] \quad (\text{M16})$$

is *not* generically destabilising in this limit. That implies that there is no generic instability towards a microphase-separated state in this model, and the transition from the disordered phase to the polar one may be continuous, without an intervening banded state. The suppression of the instability of an incipient, homogenous polar phase in an interfacial flock is a further consequence of long-range fluid interactions.

#### Appendix N: Effect of interfacial fluctuations on the ordered state

The calculations presented in the main text assumed a flat interface or surface and tacitly ignored shape fluctuations of the interface. In this supplementary section, I demonstrate that small interfacial fluctuations do not affect the ordered state. For simplicity, I will consider an immersed interface with viscosity-matched fluids above and below the interface with viscosity  $\eta$  and consider only nematic order with nematogens free to diffuse out of the interface. This can be generalised easily to all the cases considered in the article without any modification of the qualitative results [58].

The order is confined to the tangent plane and since the interfacial fluctuations are assumed to be small, I use the Monge gauge to parametrise the membrane displacement away from the  $z = 0$  plane; that is, a point on the interface is parametrised by the three-dimensional position vector  $\mathbf{R} = (x, y, h(x, y))$ ; see Fig. 1. With this parametrisation, the normal to the interface is  $\mathbf{N} = \frac{\hat{z} - \nabla_\perp h}{\sqrt{1 + (\nabla_\perp h)^2}}$ . The three-component nematic director, with in-plane order along  $\hat{x}$ , is denoted by  $\mathbf{n}(\mathbf{r}_\perp, t) \equiv (n_x, n_y, n_z) = \frac{\hat{x} + \delta \mathbf{n}}{\sqrt{1 + \delta \mathbf{n} \cdot \delta \mathbf{n}}}$ . Since the director is confined to the tangent plane,

$$\mathbf{n} \cdot \mathbf{N} = 0 = \frac{1}{\sqrt{1 + \delta \mathbf{n} \cdot \delta \mathbf{n}}} \frac{1}{\sqrt{1 + (\nabla_\perp h)^2}} [\delta n_z - \delta n_y \partial_y h - (1 + \delta n_x) \partial_x h] \implies \delta n_z \approx \partial_x h \quad (\text{N1})$$

where the final approximate equality is obtained by retaining only the linear terms. The interface fluctuations are controlled by a free energy of the form  $F_{\text{int}} = (12) \int d\mathbf{x} [\varsigma (\nabla_\perp h)^2 + \kappa (\nabla_\perp^2 h)^2]$  where  $\varsigma$  is the surface tension and  $\kappa$  is the bending modulus. Denoting  $\delta n_y = \theta$  for continuity of notation, the active force  $\propto \nabla_\perp \cdot (\mathbf{n}\mathbf{n}) = \partial_y \theta \hat{x} + \partial_x \theta \hat{y} + \partial_x^2 h \hat{z}$ , to linear order, where I have used  $\delta n_z \approx \partial_x h$ . Putting all these together, the linearised force balance equation, in the notation of Supp. C, is

$$-\eta \nabla^2 \mathbf{V} = -\nabla \Pi - \varsigma (\partial_y \theta \hat{x} + \partial_x \theta \hat{y}) \delta(z) - \left( \varsigma \partial_x^2 h + \frac{\delta F_{\text{int}}}{\delta h} \right) \hat{z} \delta(z) + \boldsymbol{\xi}^v, \quad (\text{N2})$$

while the dynamics of  $\theta$  is still described by (E1) and the equation of motion for the height fluctuations is simply  $\partial_t h = V_z|_{z=0}$ . Solving for the velocity field as in Supp. C,  $v_x = -(i\varsigma q_y^3 / 2\eta |q_\perp|^3) \theta + \bar{\xi}_x^v$  and  $v_y = -(i\varsigma q_x^3 / 2\eta |q_\perp|^3) \theta + \bar{\xi}_y^v$  which yields (E2) (ignoring, as earlier,  $\bar{\xi}_x^v$  and  $\bar{\xi}_y^v$  in comparison to  $\xi$ ) and

$$V_z(z=0) = -\frac{1}{4\eta |q_\perp|} (\varsigma q_\perp^2 + \kappa q_\perp^4 - \varsigma q_x^2) h + \bar{\xi}_z^v. \quad (\text{N3})$$

This implies that to linear order, the angular dynamics is unaffected by the height fluctuations, while the linearised equation for the height fluctuations is

$$\partial_t h = -\frac{1}{4\eta|q_\perp|}(\varsigma q_\perp^2 + \kappa q_\perp^4 - \zeta q_x^2)h + \bar{\xi}_z^v, \quad (\text{N4})$$

i.e., activity yields an effective surface tension-like term for fluctuations along the ordering direction. Therefore, a flat interface is destabilised for  $\zeta > \varsigma$  i.e. when *extensile* activity is greater than the surface tension. In that case, the interface may have an undulated conformation as in [34]. This situation is likely to be realised for an ordered phase on a self-assembled membrane. Conversely, when  $\zeta < \varsigma$ , the flat interface results described in this article are realised even in this fluctuating context. In this case, the static structure factor of height fluctuations is

$$\langle |h(\mathbf{q}_\perp, t)|^2 \rangle = \frac{\Delta^v}{\eta(\varsigma q_\perp^2 + \kappa q_\perp^4 - \zeta q_x^2)}. \quad (\text{N5})$$

This implies that small fluctuations of an interface or a boundary cannot modify the conclusions regarding interfacial order described in this article. In particular, nematic or polar phases associated with interfaces are likely to be realised even when the interface does not remain perfectly flat.

---

\* nyomaitra07@gmail.com

- [1] R. V. Craster, O. K. Matar and D. T. Papageorgiou, *Breakup of surfactant-laden jets above the critical micelle concentration*, J. Fluid Mech. **629**, 195 (2009). doi:10.1017/S0022112009006533
- [2] A. Kalogirou and M. G. Blyth, *The role of soluble surfactants in the linear stability of two-layer flow in a channel*, J. Fluid Mech. **873**, 18 (2019). doi:10.1017/jfm.2019.392
- [3] S. J. Kole, G. P. Alexander, S. Ramaswamy and A. Maitra, *Layered chiral active matter: beyond odd elasticity*, Phys. Rev. Lett. **126**, 248001 (2021). doi:10.1103/PhysRevLett.126.248001
- [4] A. Tiribocchi, R. Wittkowski, D. Marenduzzo, and M.E. Cates, *Active model H: scalar active matter in a momentum-conserving fluid*, Phys. Rev. Lett. **115**, 188302 (2015). doi:10.1103/PhysRevLett.115.188302.
- [5] R. Singh and M.E. Cates, *Hydrodynamically interrupted droplet growth in scalar active matter*, Phys. Rev. Lett. **123**, 148005 (2019). doi:10.1103/PhysRevLett.123.148005
- [6] R. A. Simha, S. Ramaswamy, *Hydrodynamic fluctuations and instabilities in ordered suspensions of self-propelled particles*, Phys. Rev. Lett. **89**, 058101 (2002). doi:10.1103/PhysRevLett.89.058101
- [7] R. Alert, J-F. Joanny, J. Casademunt, *Active turbulence*, arXiv:2104.02122 (2021).
- [8] P. T. Underhill, J. P. Hernandez-Ortiz and M. D. Graham, *Diffusion and spatial correlations in suspensions of swimming particles*, Phys. Rev. Lett. **100**, 248101 (2008). doi:10.1103/PhysRevLett.100.248101
- [9] P. G. Saffman and M. Delbrück, *Brownian motion in biological membranes*, Proc. Natl. Acad. Sci. USA **72**, 3111 (1975). doi:10.1073/pnas.72.8.3111
- [10] A. Maitra and R. Voituriez, *Enhanced orientational ordering induced by an active yet isotropic bath*, Phys. Rev. Lett. **124**, 048003 (2020). doi:10.1103/PhysRevLett.124.048003
- [11] T. J. Sluckin, A. Poniewierski, *Novel surface phase transition in nematic liquid crystals: Wetting and the Kosterlitz-Thouless transition*, Phys. Rev. Lett. **55**, 2907 (1985). doi:10.1103/PhysRevLett.55.2907
- [12] J. Toner, *Birth, death, and flight: A theory of Malthusian flocks*, Phys. Rev. Lett. **108**, 088102 (2012). doi:10.1103/PhysRevLett.108.088102
- [13] M. D. Khandkar and M. Barma, *Orientational correlations and the effect of spatial gradients in the equilibrium steady state of hard rods in two dimensions: A study using deposition-evaporation kinetics*, Phys. Rev. E **72**, 051717 (2005). doi:10.1103/PhysRevE.72.051717
- [14] M.C. Marchetti, J-F. Joanny, S. Ramaswamy, T.B. Liverpool, J. Prost, M. Rao, and R. A. Simha, *Hydrodynamics of soft active matter*, Rev. Mod. Phys. **85**, 1143 (2013). doi:10.1103/RevModPhys.85.1143
- [15] D. Marenduzzo, E. Orlandini, M. E. Cates, and J. M. Yeomans, *Steady-state hydrodynamic instabilities of active liquid crystals: Hybrid lattice Boltzmann simulations*, Phys. Rev. E **76**, 031921 (2007). doi:10.1103/PhysRevE.76.031921
- [16] A. P. Solon, Y. Fily, A. Baskaran, M. E. Cates, Y. Kafri, M. Kardar and J. Tailleur, *Pressure is not a state function for generic active fluids*, Nat. Phys. **11**, 673 (2015). doi:10.1038/nphys3377
- [17] J. Toner, Y. Tu, and S. Ramaswamy, *Hydrodynamics and phases of flocks*, Ann. Phys. **318**, 170 (2005). doi:10.1016/j.aop.2005.04.011
- [18] J. Toner and Y. Tu, *Long-range order in a two-dimensional dynamical XY model: How Birds Fly Together*, Phys. Rev. Lett. **75**, 4326 (1995). doi:10.1103/PhysRevLett.75.4326
- [19] J. Toner, *Reanalysis of the hydrodynamic theory of fluid, polar-ordered flocks*, Phys. Rev. E **86**, 031918 (2013). doi:10.1103/PhysRevE.86.031918
- [20] A. Maitra, P. Srivastava, M. C. Marchetti, S. Ramaswamy and M. Lenz, *Swimmer suspensions on substrates: anomalous stability and long-range order*, Phys. Rev. Lett. **124**, 028002 (2020). doi:10.1103/PhysRevLett.124.028002

- [21] L. Giomi, M. C. Marchetti and T. B. Liverpool, *Complex spontaneous flows and concentration banding in active polar films*, Phys. Rev. Lett. **101**, 198101 (2008). doi:10.1103/PhysRevLett.101.198101
- [22] P. G. de Gennes, J. Prost, *The Physics of Liquid Crystals (second edition)*, Clarendon, Oxford (1993)
- [23] S. Ramaswamy, R. A. Simha, J. Toner, *Active nematics on a substrate: giant number fluctuations and long-time tails*, Europhys. Lett. **62**, 196 (2003). doi:10.1209/epl/i2003-00346-7
- [24] A. Maitra, P. Srivastava, M. C. Marchetti, J. S. Lintuvuori, S. Ramaswamy and M. Lenz, *A nonequilibrium force can stabilize 2D active nematics*, Proc. Natl. Acad. Sci. USA **115**, 6934 (2018). doi:10.1073/pnas.1720607115
- [25] W. Kung, M. C. Marchetti and K. Saunders, *Hydrodynamics of polar liquid crystals*, Phys. Rev. E **73**, 031708 (2006). doi:10.1103/PhysRevE.73.031708
- [26] B. Martínez-Prat J. Ignés-Mullol, J. Casademunt and Francesc Sagués, *Selection mechanism at the onset of active turbulence*, Nat. Phys. **15**, 362 (2019). doi:10.1038/s41567-018-0411-6
- [27] T. Gao, R. Blackwell, M. A. Glaser, M. D. Betterton and M. J. Shelley, *Multiscale modeling and simulation of microtubule-motor-protein assemblies*, Phys. Rev. E **92**, 062709 (2015). doi:10.1103/PhysRevE.92.062709
- [28] T. Gao, R. Blackwell, M. A. Glaser, M. D. Betterton and M. J. Shelley, *Multiscale polar theory of microtubule and motor-protein assemblies*, Phys. Rev. Lett. **114**, 048101 (2015). doi:10.1103/PhysRevLett.114.048101
- [29] B. I. Halperin, *On the Hohenberg-Mermin-Wagner theorem and its limitations*, J. Stat. Phys. **175**, 521 (2019). doi:10.1007/s10955-018-2202-y
- [30] P. M. Chaikin, T. C. Lubensky, *Principles of Condensed Matter Physics*, Cambridge University Press (2000)
- [31] S. Mishra, R. A. Simha and S. Ramaswamy, *A dynamic renormalization group study of active nematics*, J. Stat. Mech. P02003 (2010). doi:10.1088/1742-5468/2010/02/P02003
- [32] D. R. Nelson and R. A. Pelcovits, *Momentum-shell recursion relations, anisotropic spins, and liquid crystals in  $2 + \epsilon$  dimensions*, Phys. Rev. B **16**, 2191 (1977). doi:10.1103/PhysRevB.16.2191
- [33] S. Shankar, S. Ramaswamy and M. C. Marchetti, *Low-noise phase of a two-dimensional active nematic system*, Phys. Rev. E **97**, 012707 (2018). doi:10.1103/PhysRevE.97.012707
- [34] A. Senoussi, S. Kashida, R. Voituriez, J. C. Galas, A. Maitra, and A. Estevez-Torres, *Tunable corrugated patterns in an active nematic sheet*, Proc. Natl. Acad. Sci. U.S.A. **116**, 22464 (2019). doi:10.1073/pnas.1912223116
- [35] B. Martínez-Prat, R. Alert, F. Meng, J. Ignés-Mullol, J.-F. Joanny, J. Casademunt, R. Golestanian, and F. Sagués, *Scaling regimes of active turbulence with external dissipation*, Phys. Rev. X **11**, 031065 (2021). doi:10.1103/PhysRevX.11.031065
- [36] R. Alert, J.-F. Joanny, J. Casademunt, *Universal scaling of active nematic turbulence*, Nat. Phys. **16**, 682 (2020). doi:10.1038/s41567-020-0854-4
- [37] G. Duclos, R. Adkins, D. Banerjee, M. S. E. Peterson, M. Varghese, I. Kolvin, A. Baskaran, R. A. Pelcovits, T. R. Powers, A. Baskaran, F. Toschi, M. F. Hagan, S. J. Streichan, V. Vitelli, D. A. Beller and Z. Dogic, *Topological structure and dynamics of three-dimensional active nematics*, Science **367**, 1120 (2020). doi:10.1126/science.aaz4547
- [38] I. Dzyaloshinskii, *Theory of disclinations in liquid crystals*, Sov. Phys. JETP **31**, 773 (1970).
- [39] S. Shankar, S. Ramaswamy, M. C. Marchetti and M. J. Bowick, *Defect unbinding in active nematics*, Phys. Rev. Lett. **121**, 10800 (2018). doi:10.1103/PhysRevLett.121.108002
- [40] L. M. Pismen, *Dynamics of defects in an active nematic layer*, Phys. Rev. E **88**, 050502 (2013). doi:10.1103/PhysRevE.88.050502
- [41] L. M. Pismen and F. Sagués, *Viscous dissipation and dynamics of defects in an active nematic interface*, Eur. Phys. J. E **40**, 92 (2017). doi:10.1140/epje/i2017-11582-8
- [42] L. Giomi, M. J. Bowick, P. Mishra, R. Sknepnek and M. C. Marchetti, *Defect dynamics in active nematics*, Philos. Trans. Royal Soc. A **372**, 20130365 (2014). doi:10.1098/rsta.2013.0365
- [43] V. Narayan, S. Ramaswamy and N. Menon, *Long-lived giant number fluctuations in a swarming granular nematic*, Science **317**, 105 (2007). doi:10.1126/science.1140414
- [44] F. Vafa, M. J. Bowick, M. C. Marchetti and B. I. Shraiman, *Multi-defect dynamics in active nematics*, arXiv: 2007.02947 (2020)
- [45] A. Maitra, M. Lenz, and R. Voituriez, *Chiral Active Hexatics: Giant Number Fluctuations, Waves, and Destruction of Order*, Phys. Rev. Lett. **125**, 238005 (2020). doi:10.1103/PhysRevLett.125.238005
- [46] S. V. Maleev, *Dipole forces in two-dimensional and layered ferromagnets*, Sov. Phys. JETP **43**, 1240 (1976).
- [47] P. G. Maier and F. Schwabl, *Ferromagnetic ordering in the two-dimensional dipolar XY model*, Phys. Rev. B **70**, 134430 (2004). doi:10.1103/PhysRevB.70.134430
- [48] R. A. Pelcovits and B. I. Halperin, *Two-dimensional ferroelectric liquid crystals*, Phys. Rev. B **19**, 4614 (1979). doi:10.1103/PhysRevB.19.4614
- [49] L. Chen, C.-F. Lee, J. Toner, *Mapping two-dimensional polar active fluids to two-dimensional soap and one-dimensional sandblasting*, Nat. Comm **7**, 12215 (2016). doi:10.1038/ncomms12215
- [50] L. Angheluta, Z. Chen, M. C. Marchetti and M. J. Bowick, *The role of fluid flow in the dynamics of active nematic defects*, New J. Phys. **23**, 033009 (2021). doi:10.1088/1367-2630/abe8a8
- [51] D. Forster, *Microscopic theory of flow alignment in nematic liquid crystals*, Phys. Rev. Lett. **32**, 1161 (1974). doi:10.1103/PhysRevLett.32.1161
- [52] H. Stark and T. C. Lubensky, *Poisson-bracket approach to the dynamics of nematic liquid crystals*, Phys. Rev. E **67**, 061709 (2003). doi:10.1103/PhysRevE.67.061709
- [53] Usually, when interfacial layers are assumed to be incompressible, it is due to the presence of surfactants. However, large densities of active particles can make even a clean interface effectively incompressible.
- [54] H. Chaté, *Dry aligning dilute active matter*, Annu. Rev. Condens. Matter Phys. **11**, 189 (2019). doi:10.1146/annurev-

conmatphys-031119-050752

- [55] L. M. Lemma, M. M. Norton, A. M. Tayar, S. J. DeCamp, S. A. Aghvami, S. Fraden, M. F. Hagan and Z. Dogic, *Multiscale microtubule dynamics in active nematics*, Phys. Rev. Lett. **127**, 148001 (2021). doi:10.1103/PhysRevLett.127.148001
- [56] R. Chatterjee, N. Rana, R. A. Simha, P. Perlekar, and S. Ramaswamy, *Inertia drives a flocking phase transition in viscous active fluids*, Phys. Rev. X **11**, 031063 (2021). doi:10.1103/PhysRevX.11.031063
- [57] S. Ramaswamy, *The Mechanics and Statistics of Active Matter*, Annu. Rev. Condens. Matter Phys. **1**, 323 (2010). doi:10.1146/annurev-conmatphys-070909-104101
- [58] T. Bickel, *Hindered mobility of a particle near a soft interface*, Phys. Rev. E **75**, 041403 (2007). doi:10.1103/PhysRevE.75.041403
